# Supplementary material for: Robust Point Cloud Segmentation with Noisy Annotations
Source: arXiv:2212.03242 source file (2022-12-06)

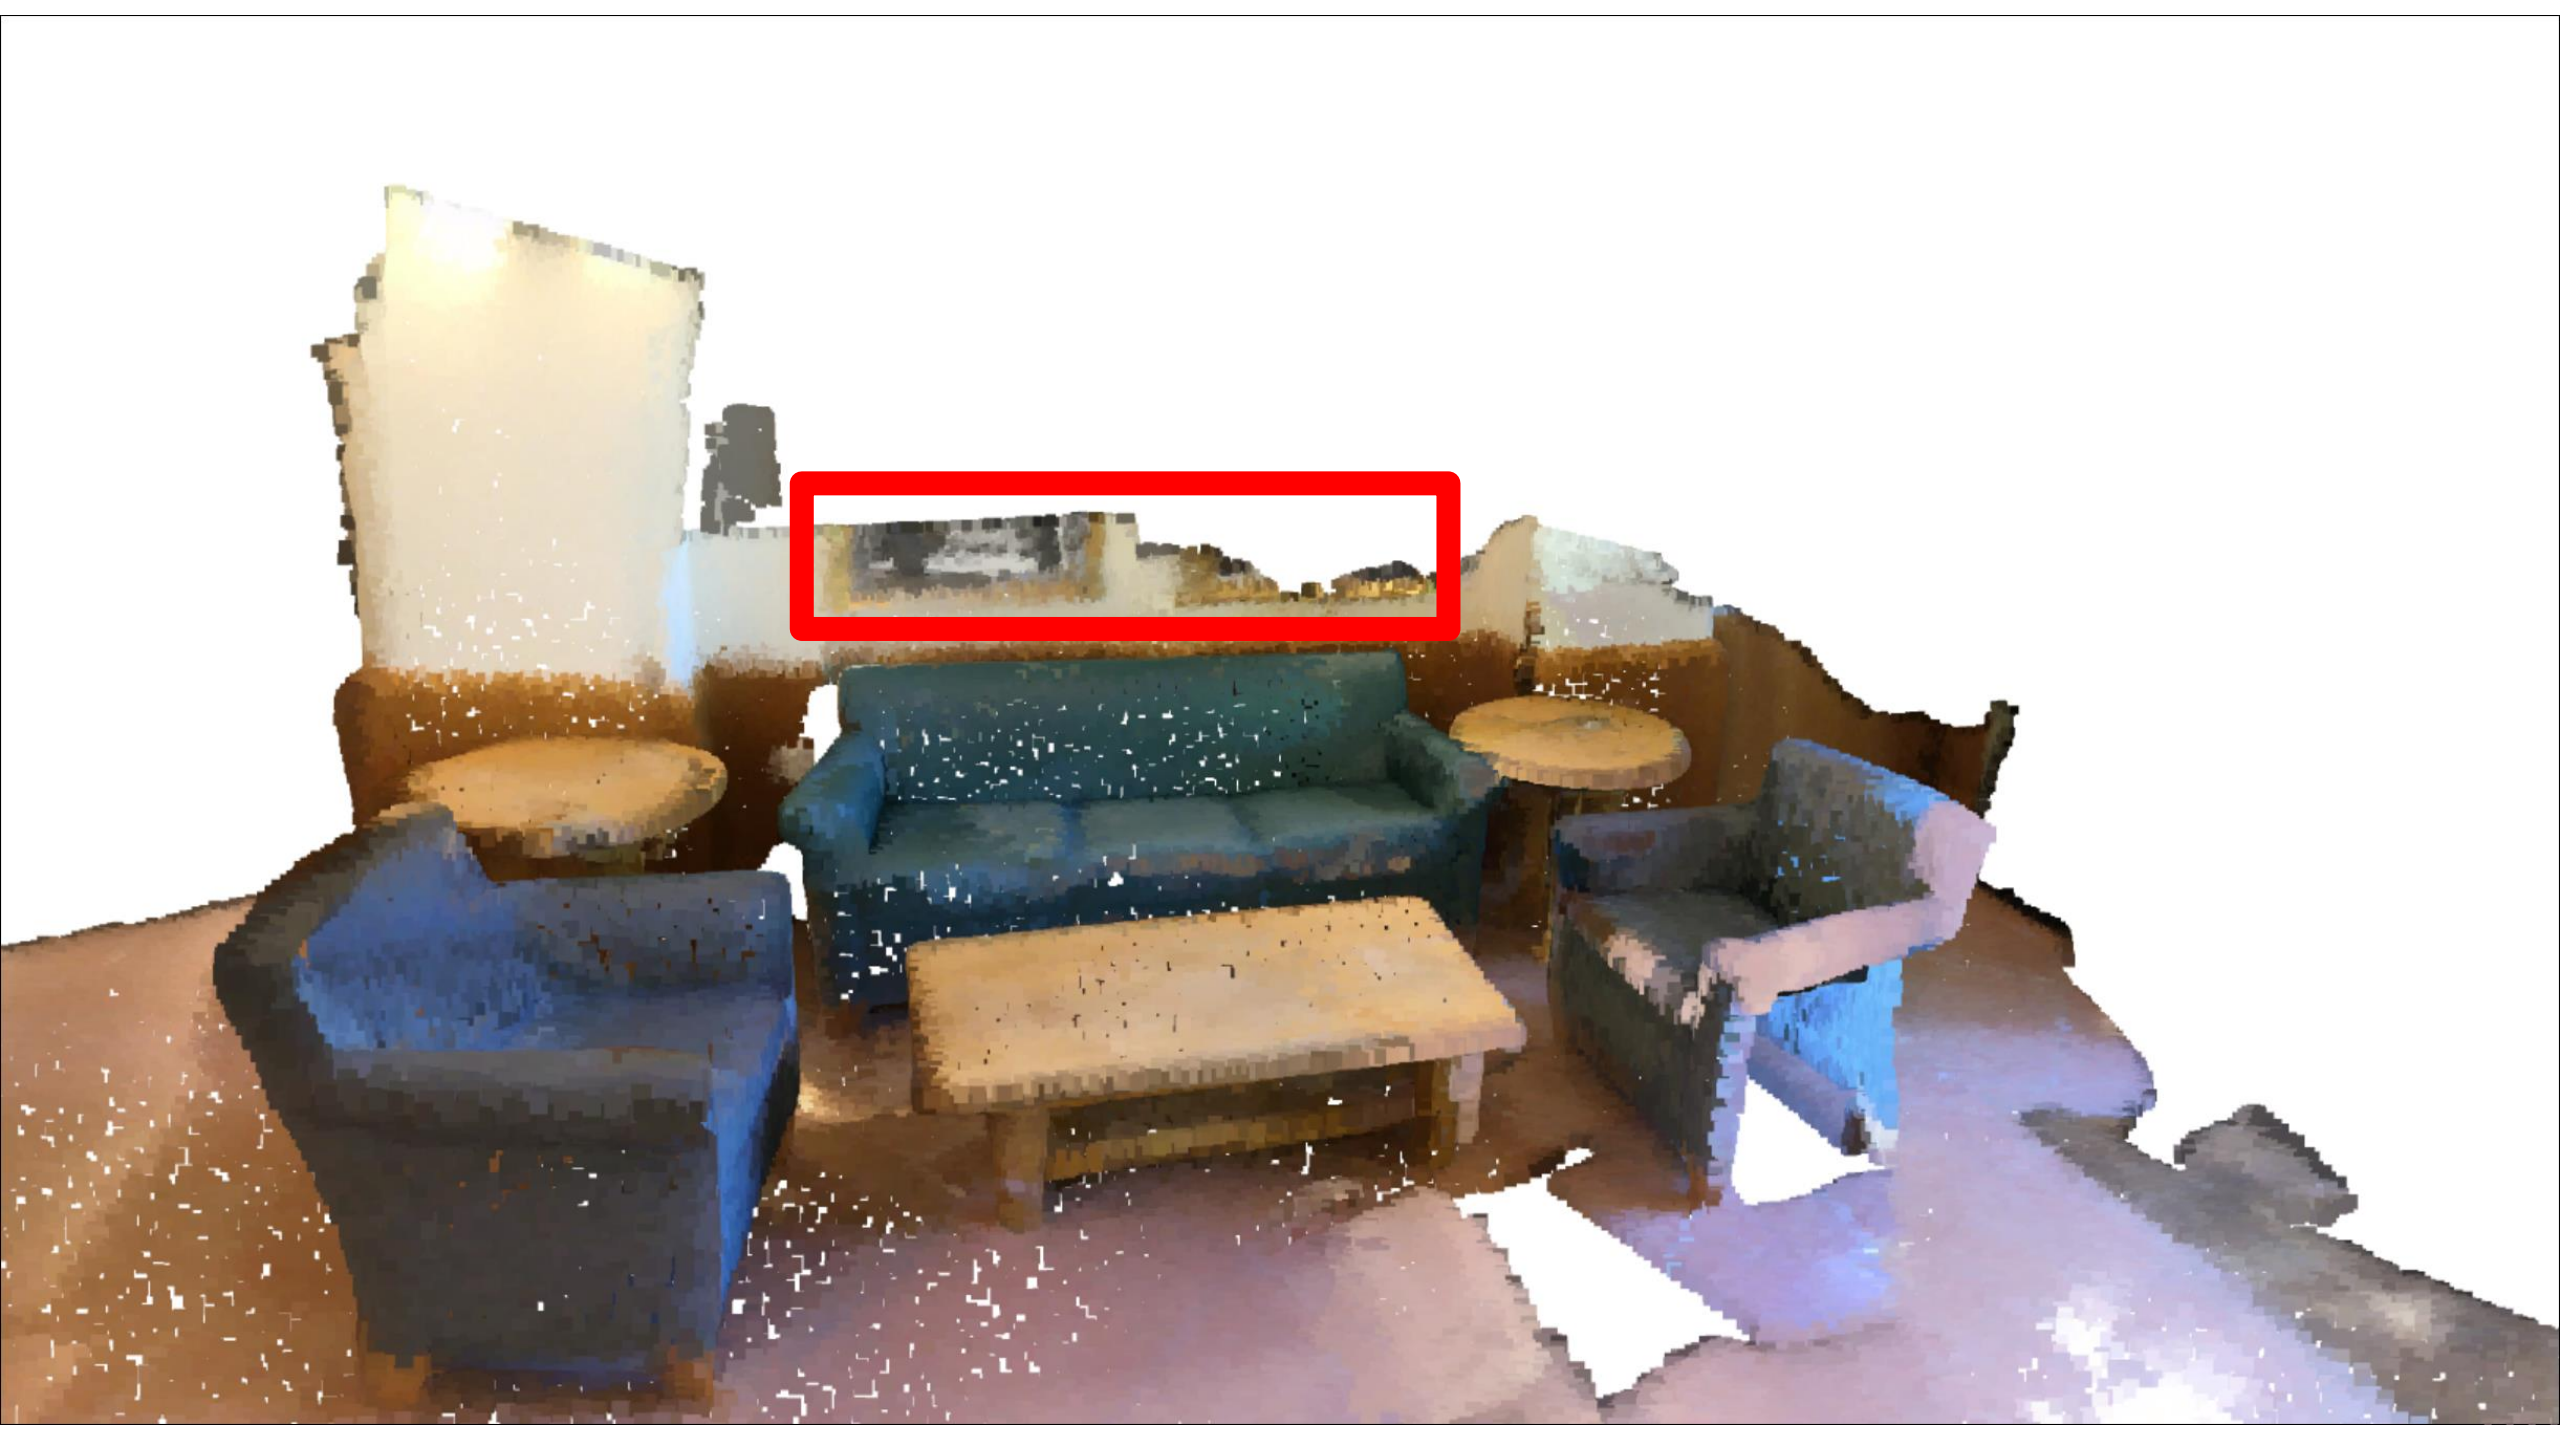

wall

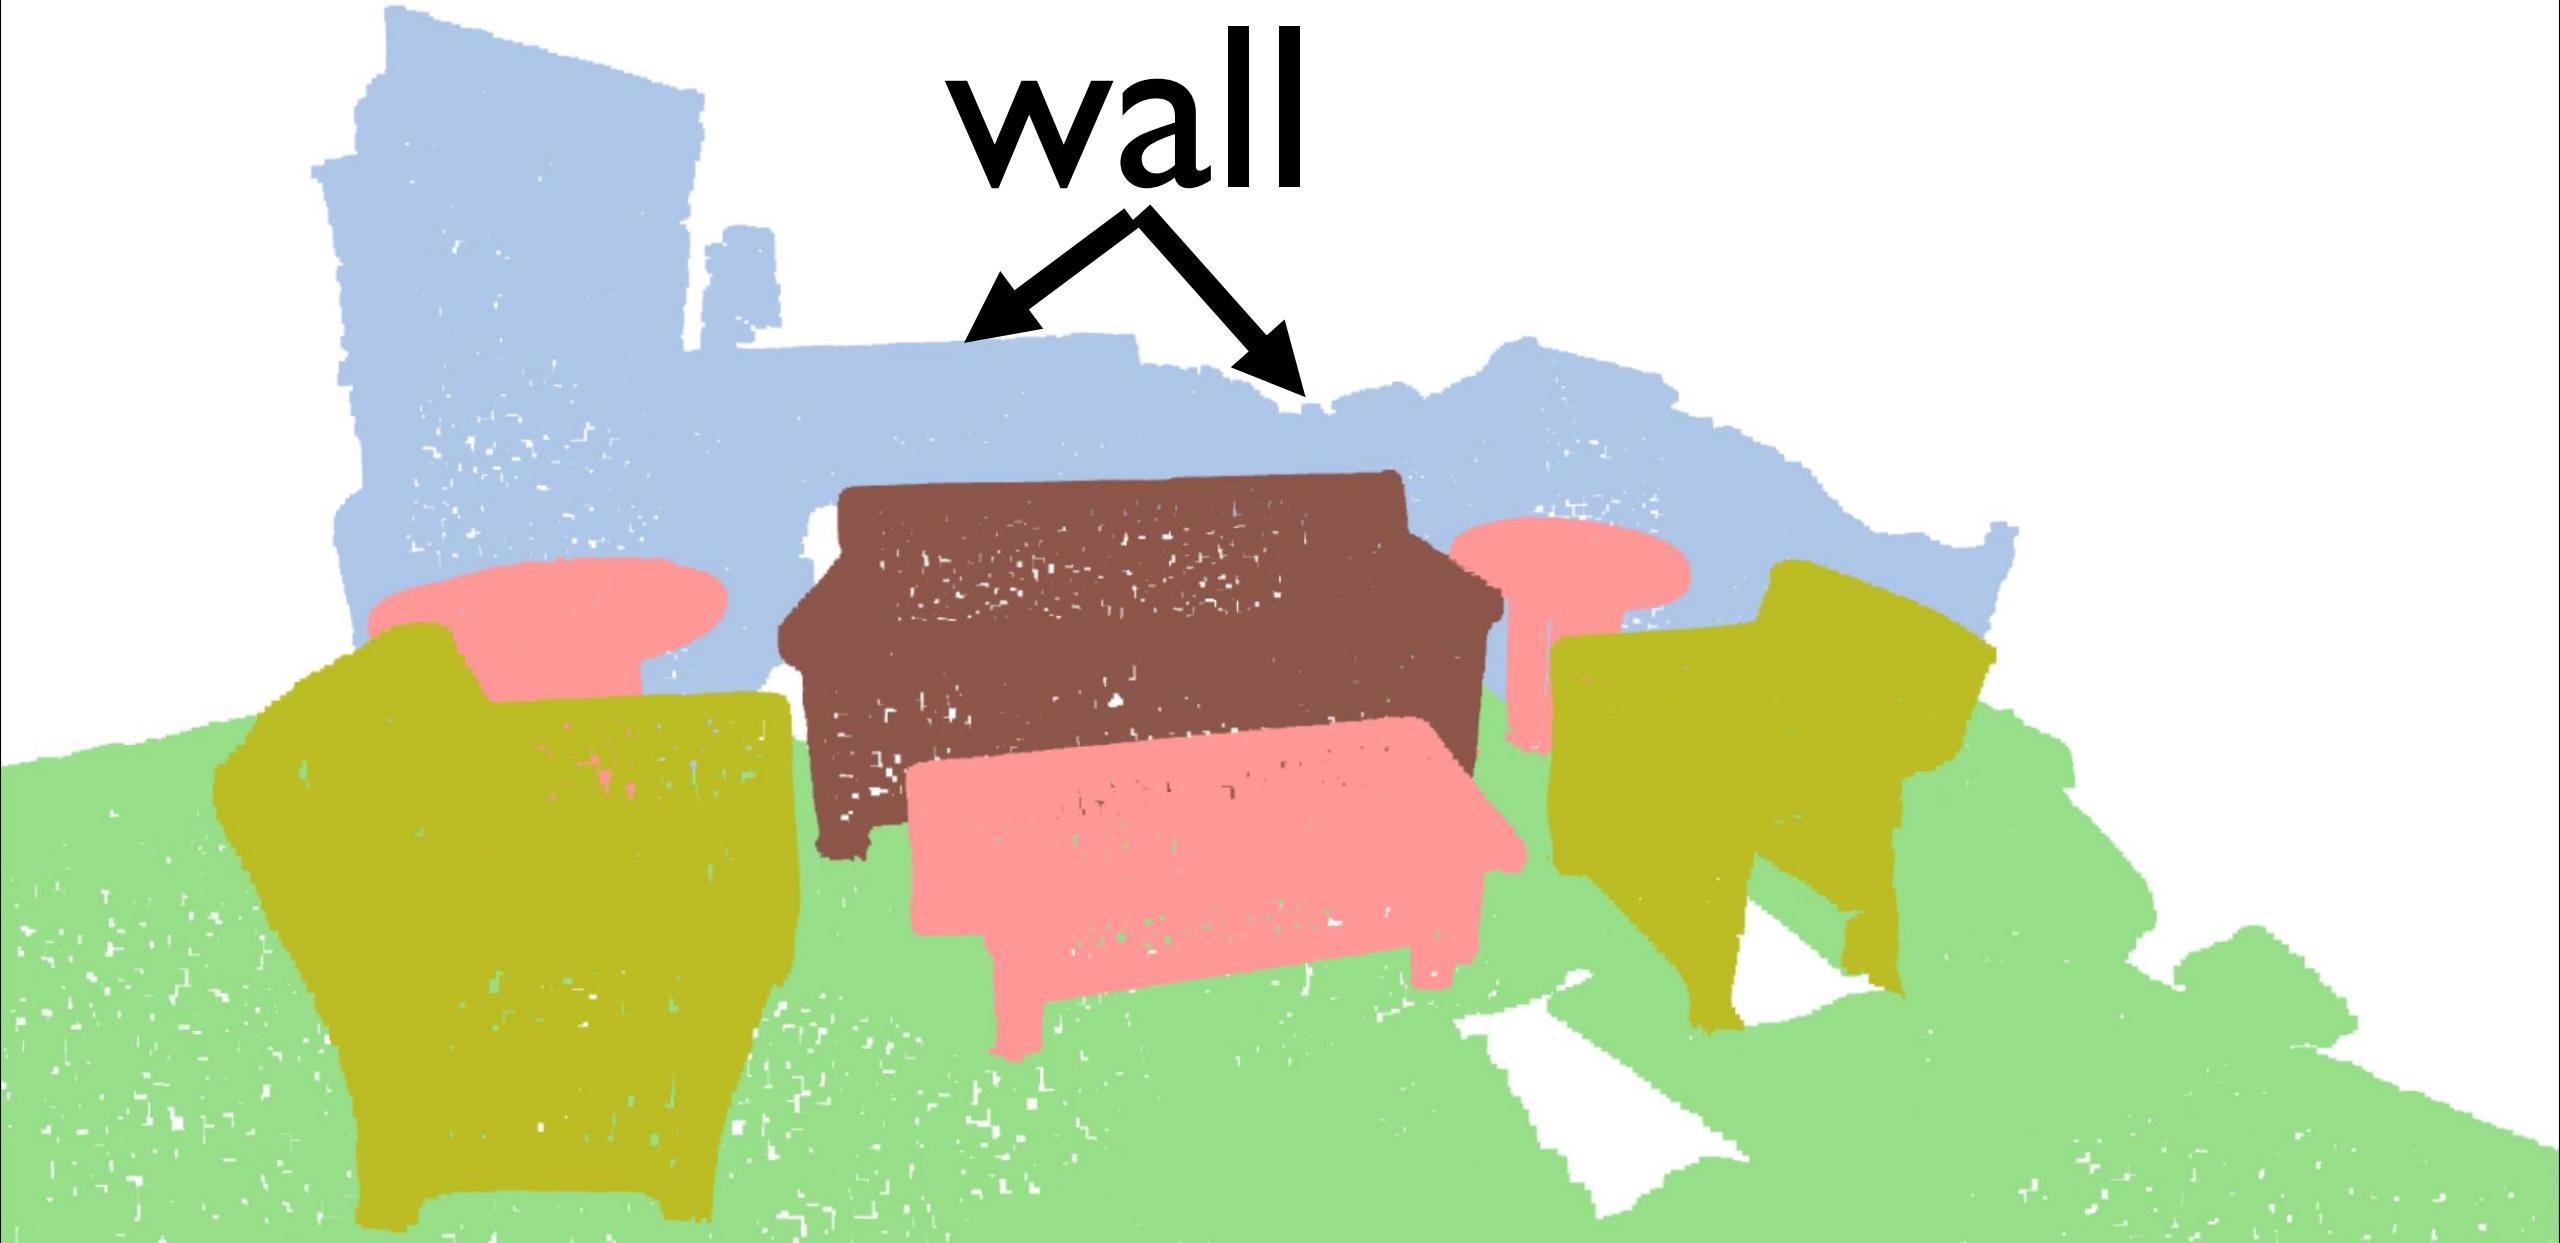

wall

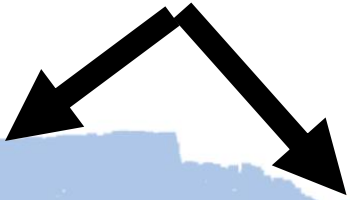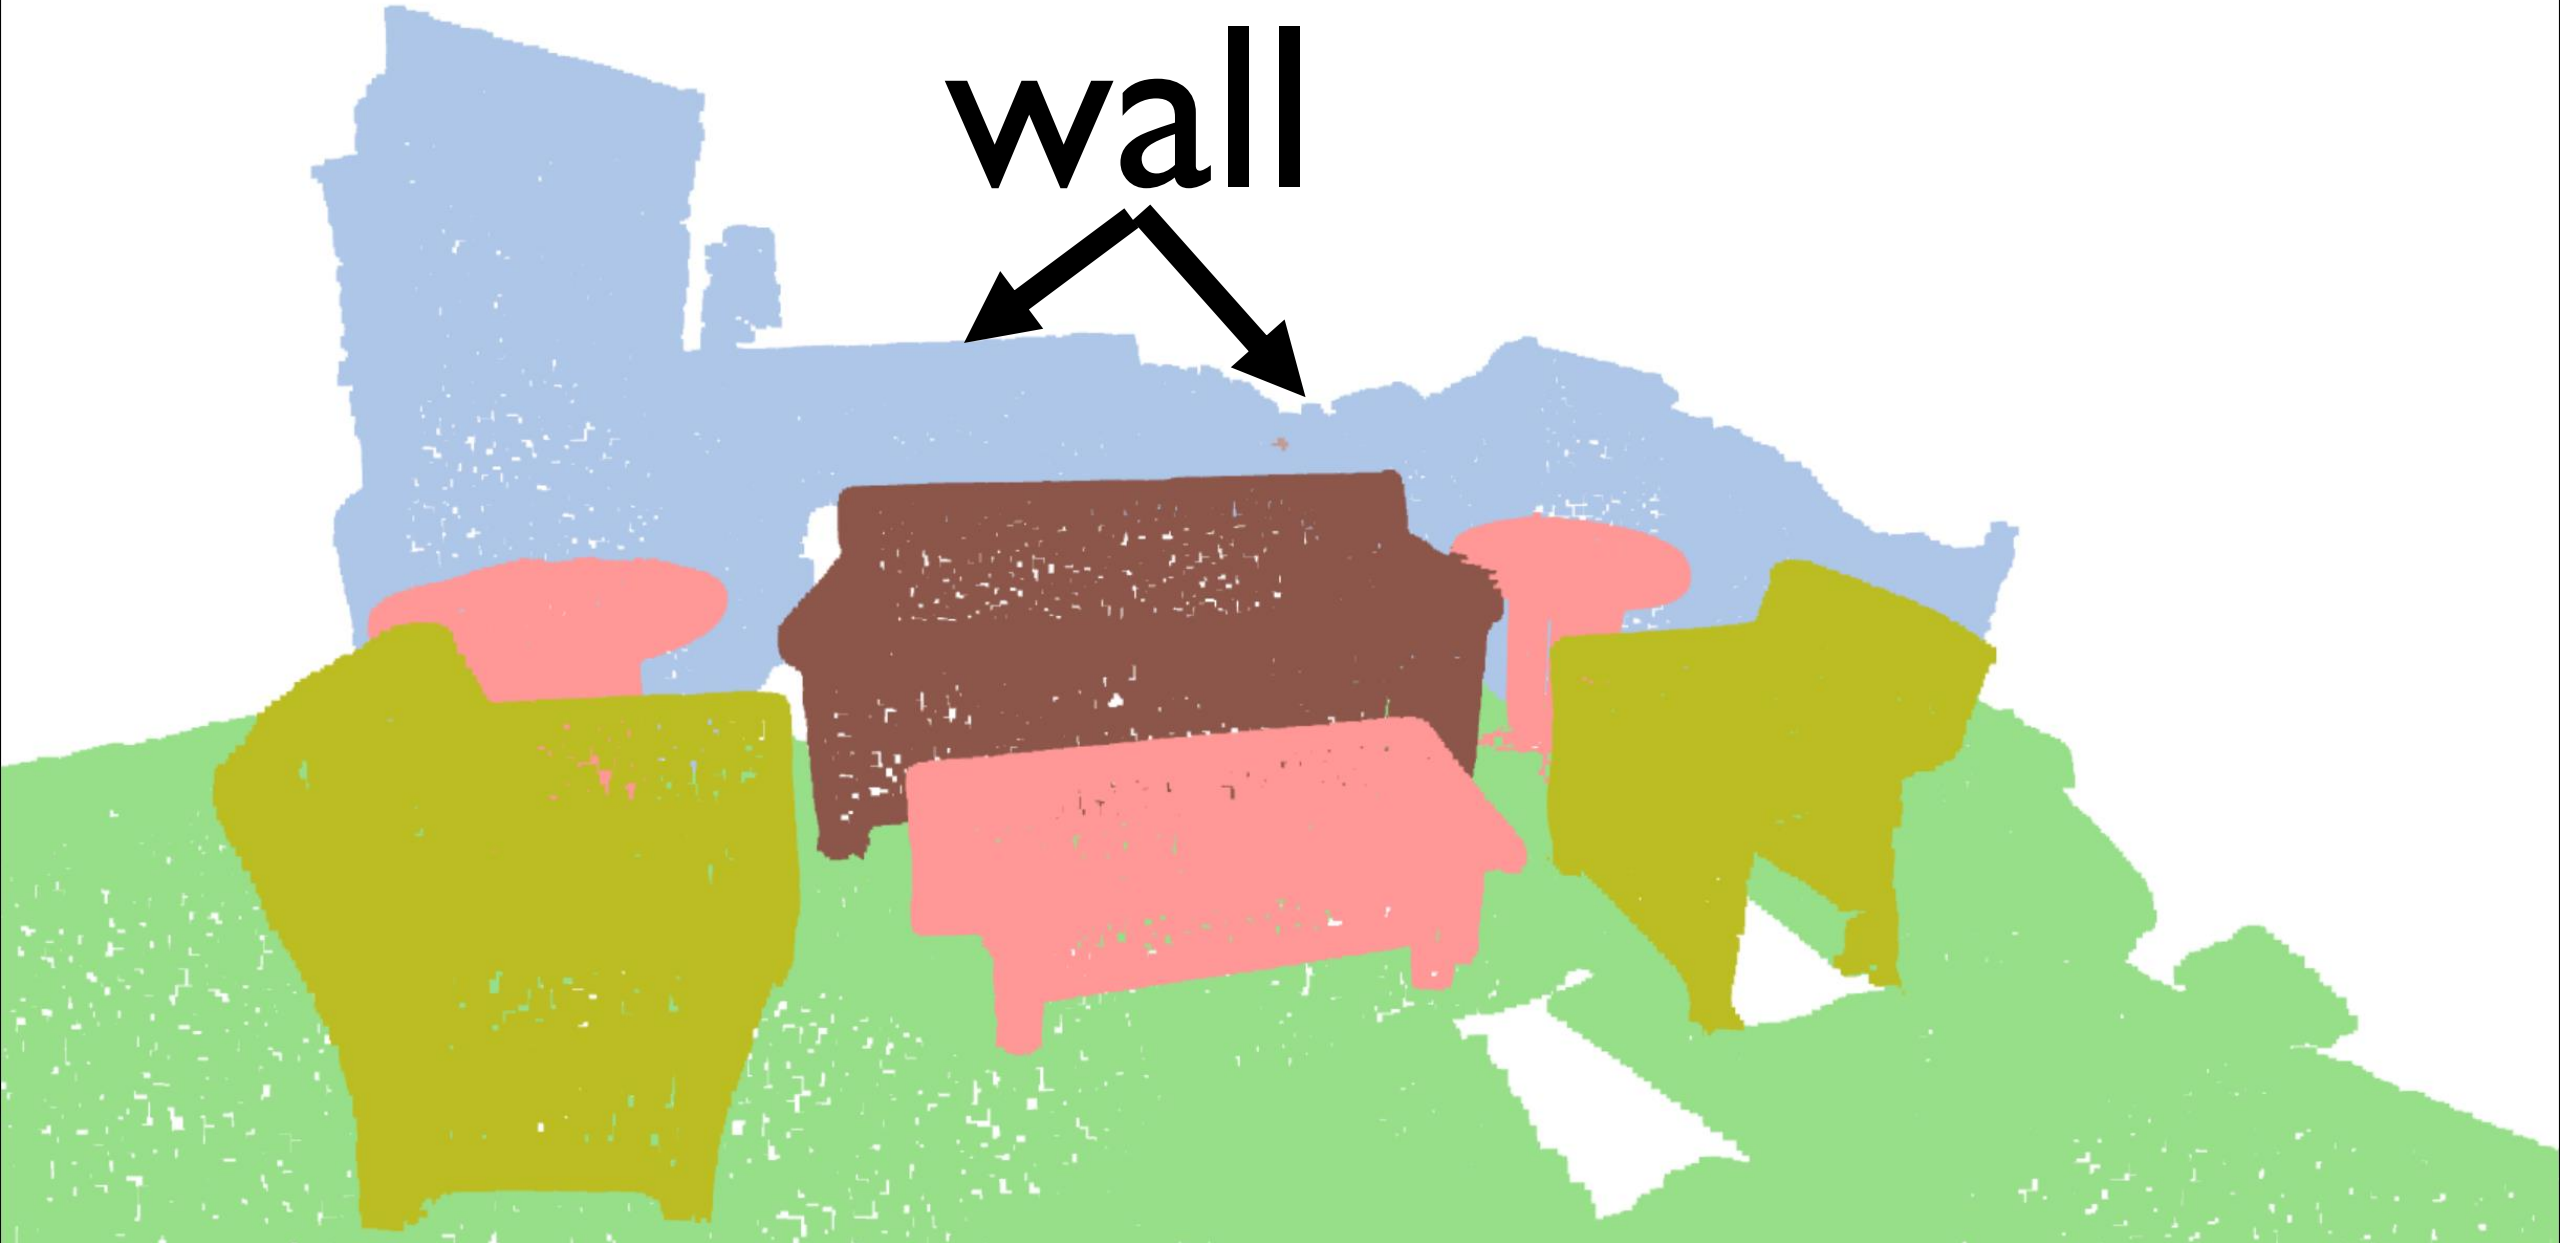

picture

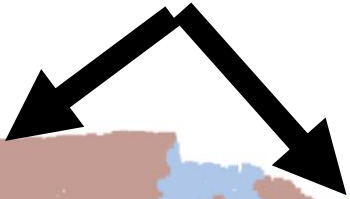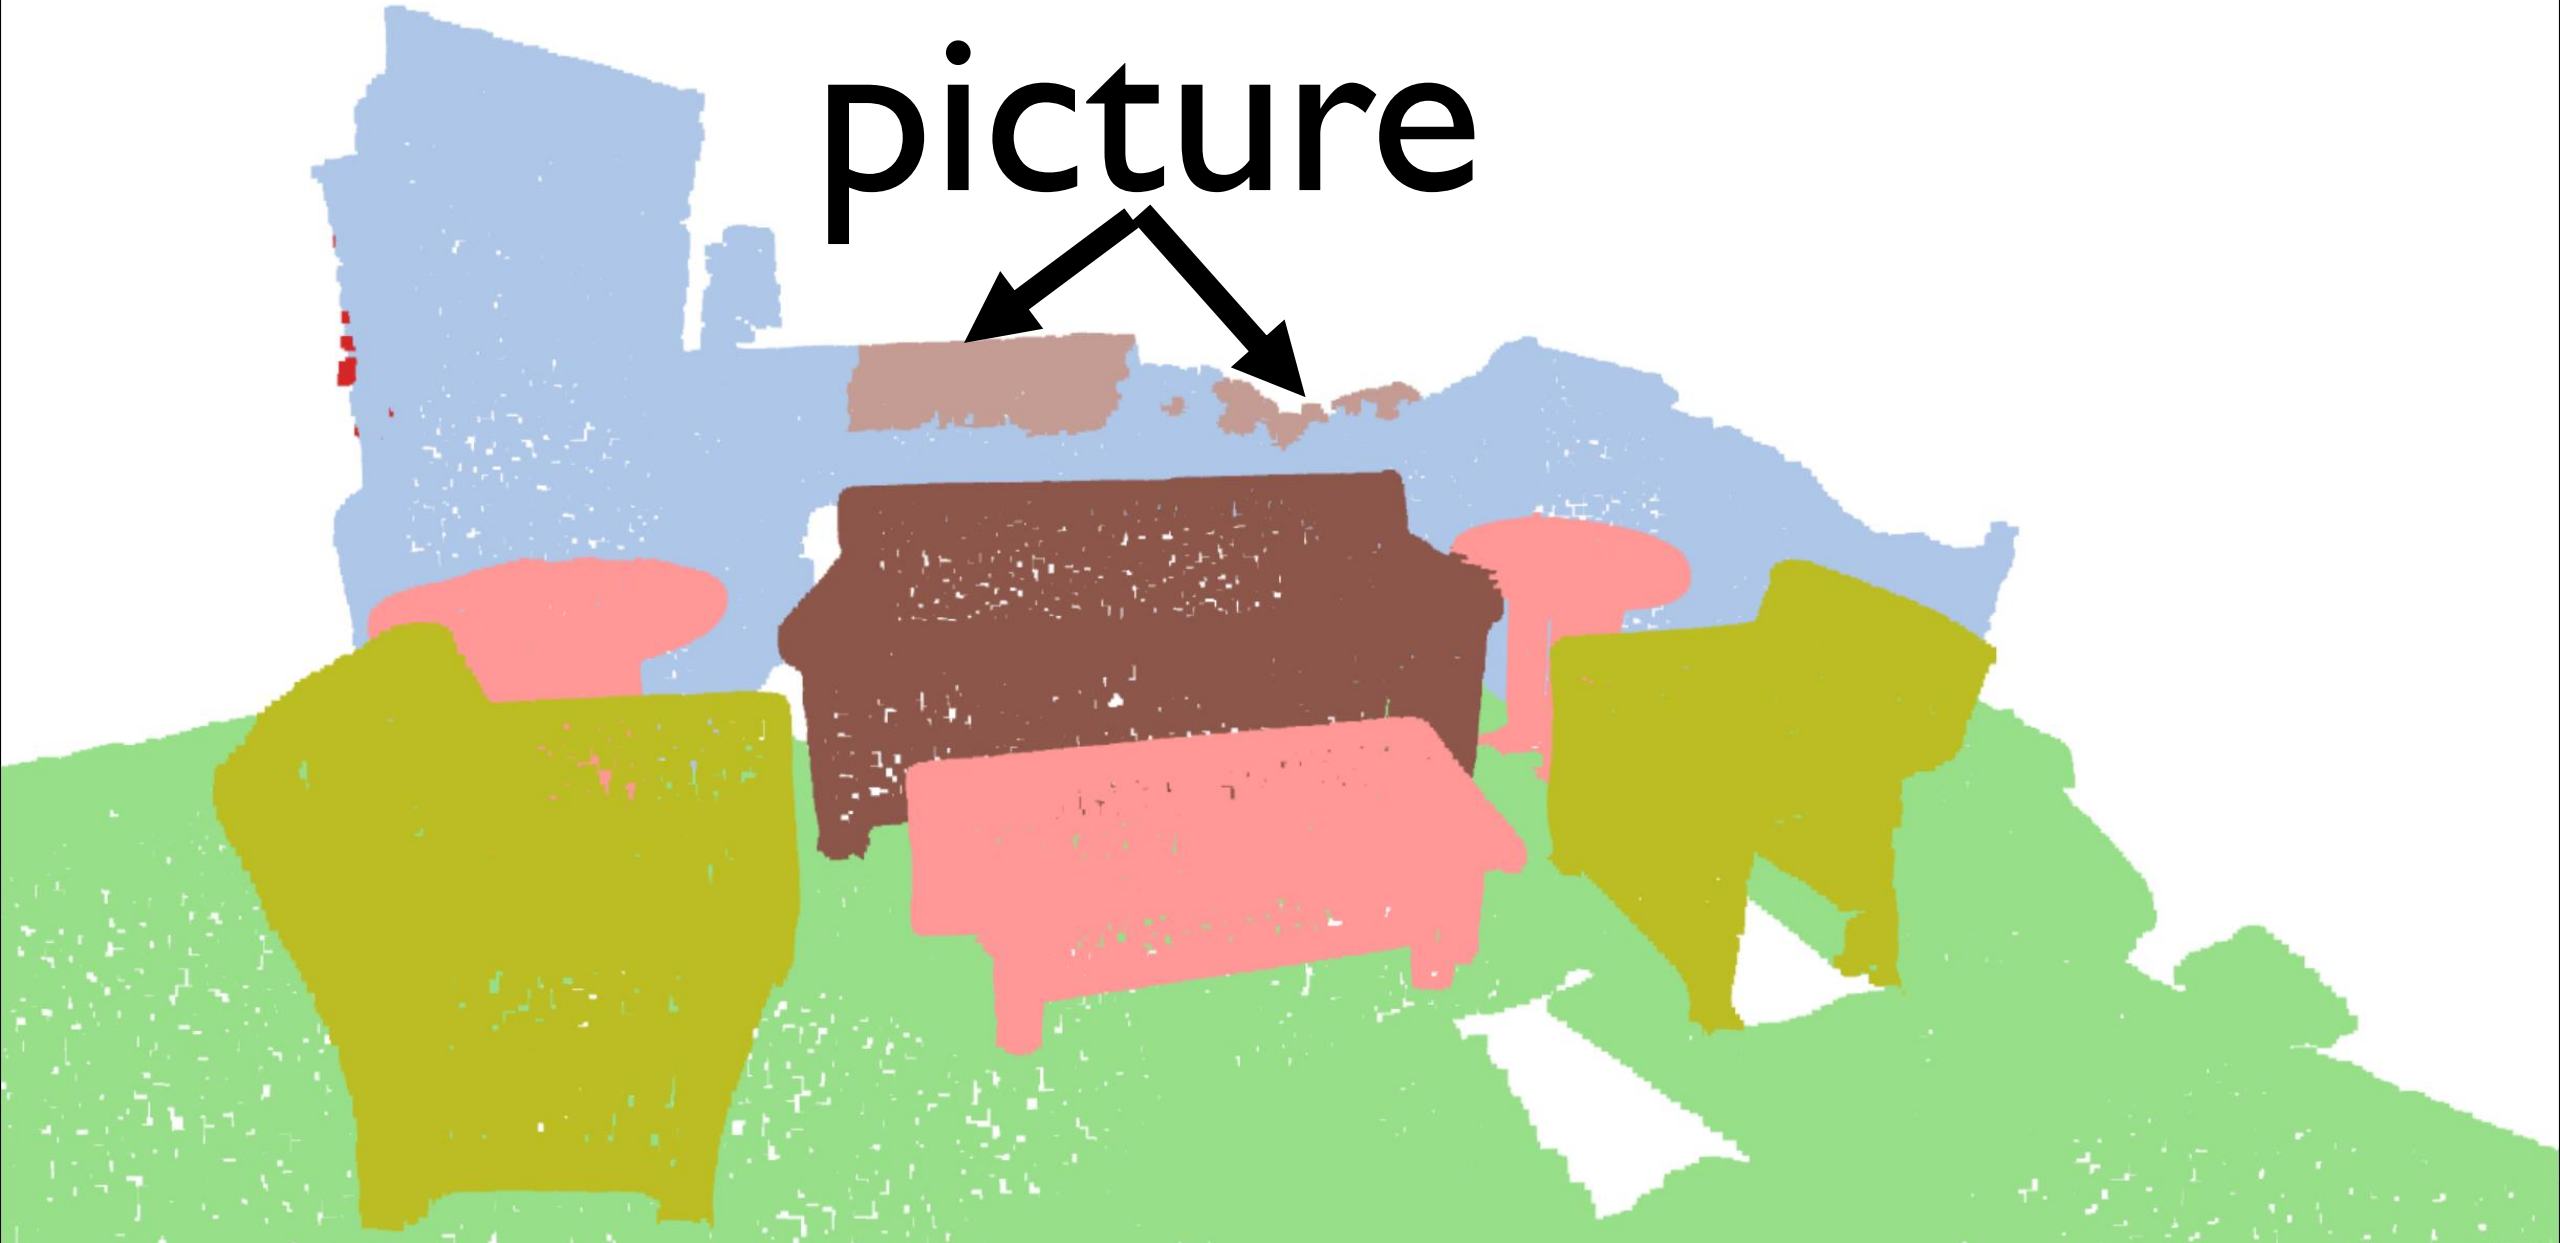

Supplement: Supplementary file 1 [file 248_oa0.9654905796051025.pdf]
