# Supplementary material for: Robust Point Cloud Segmentation with Noisy Annotations
Source: arXiv:2212.03242 source file (2022-12-06)

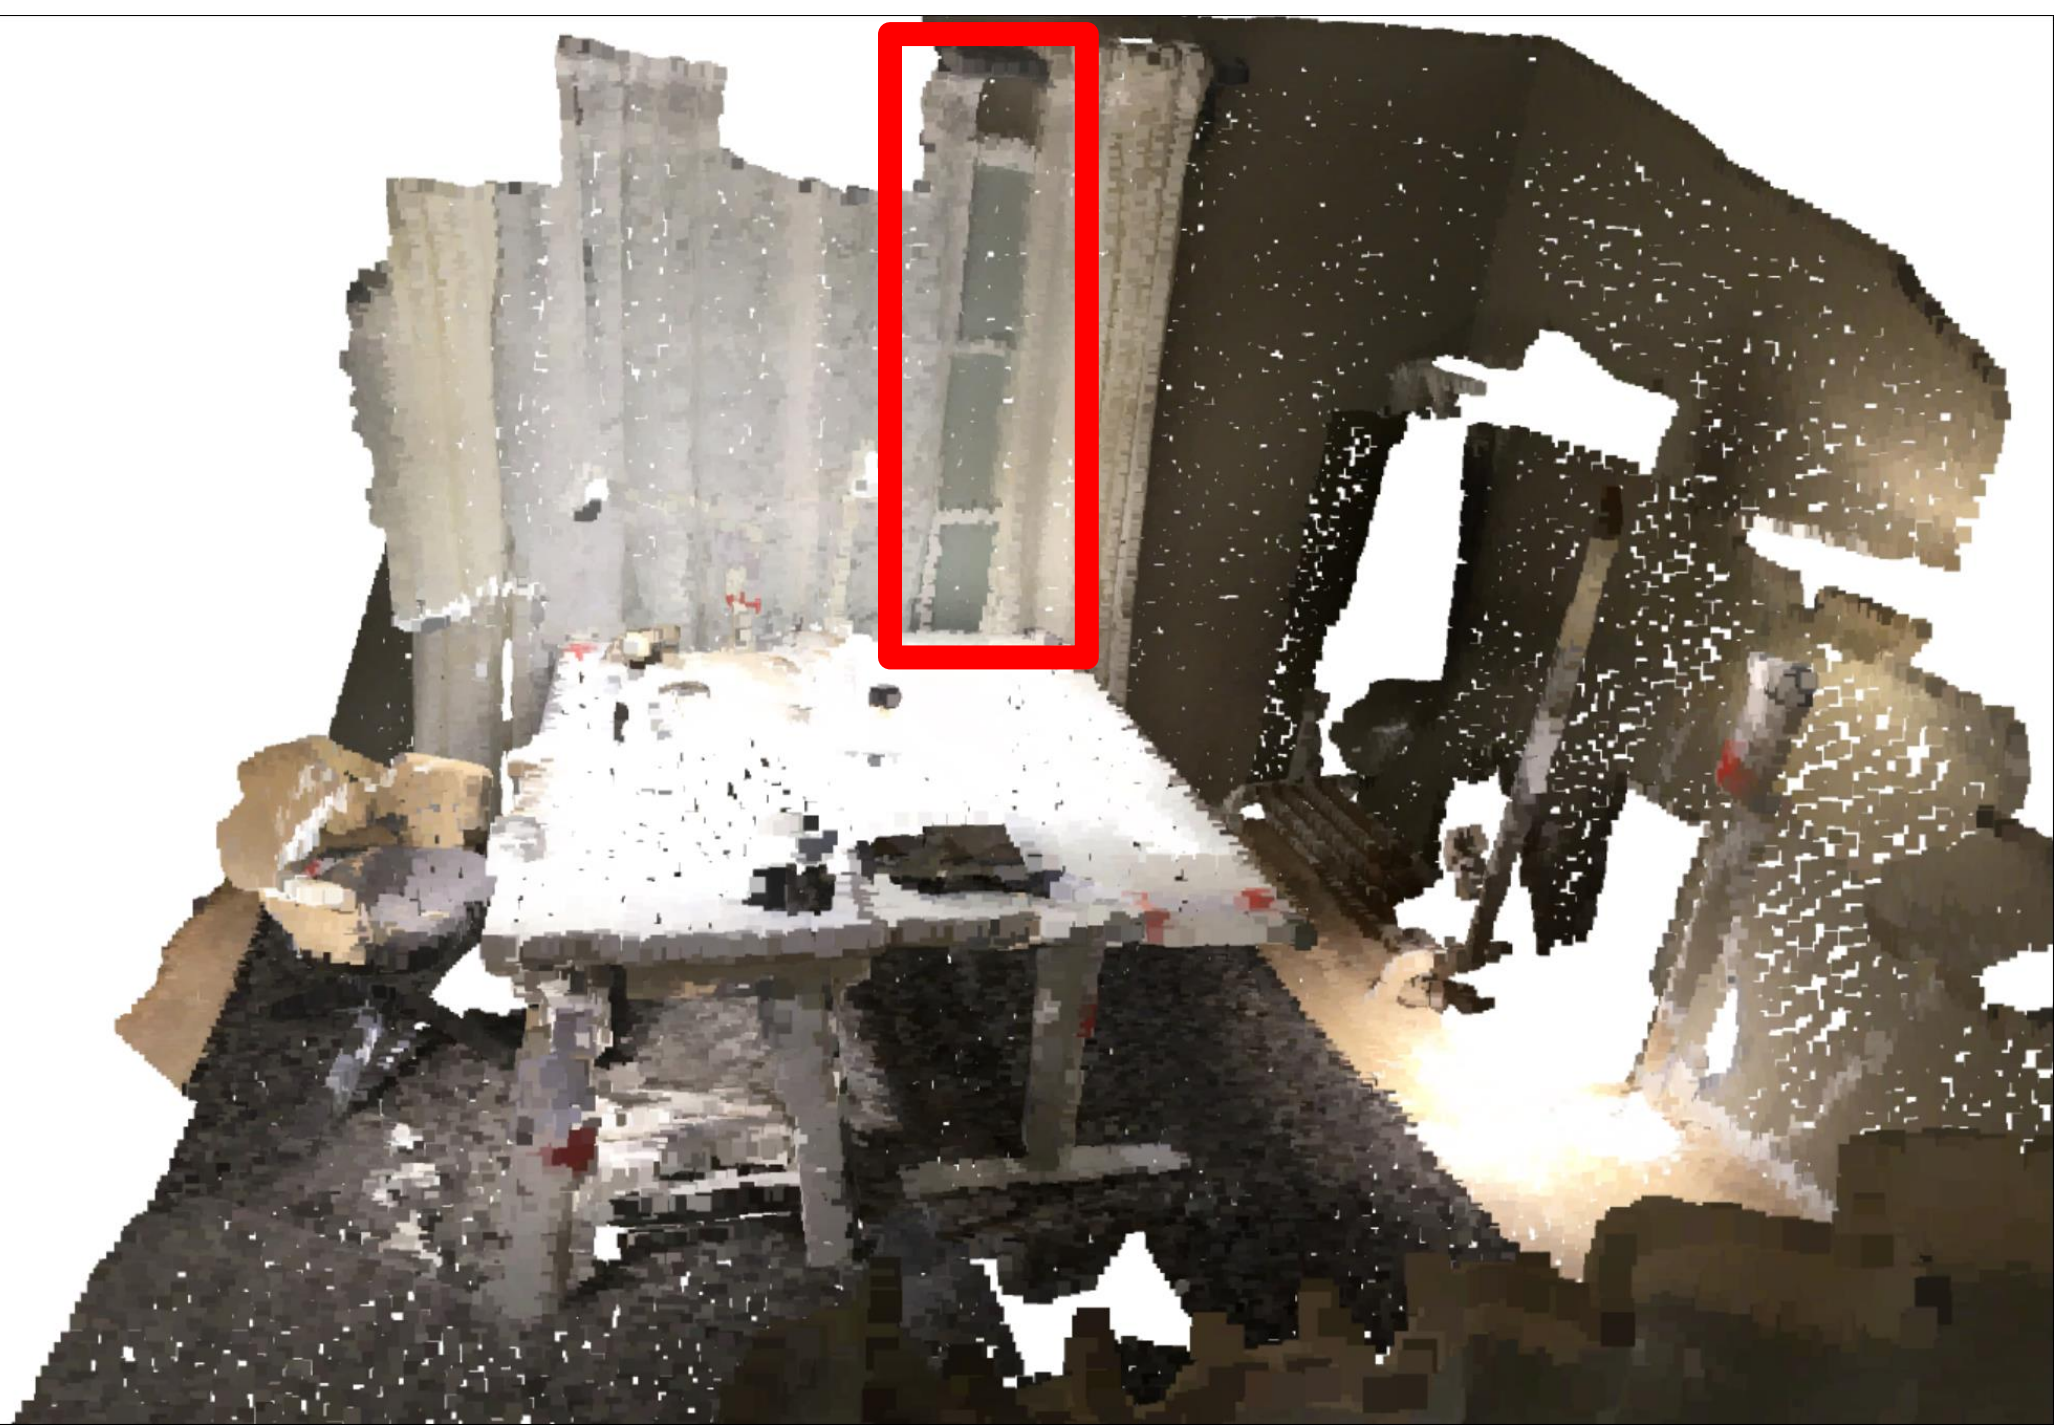

curtain

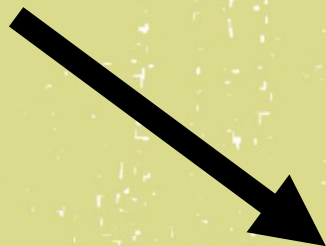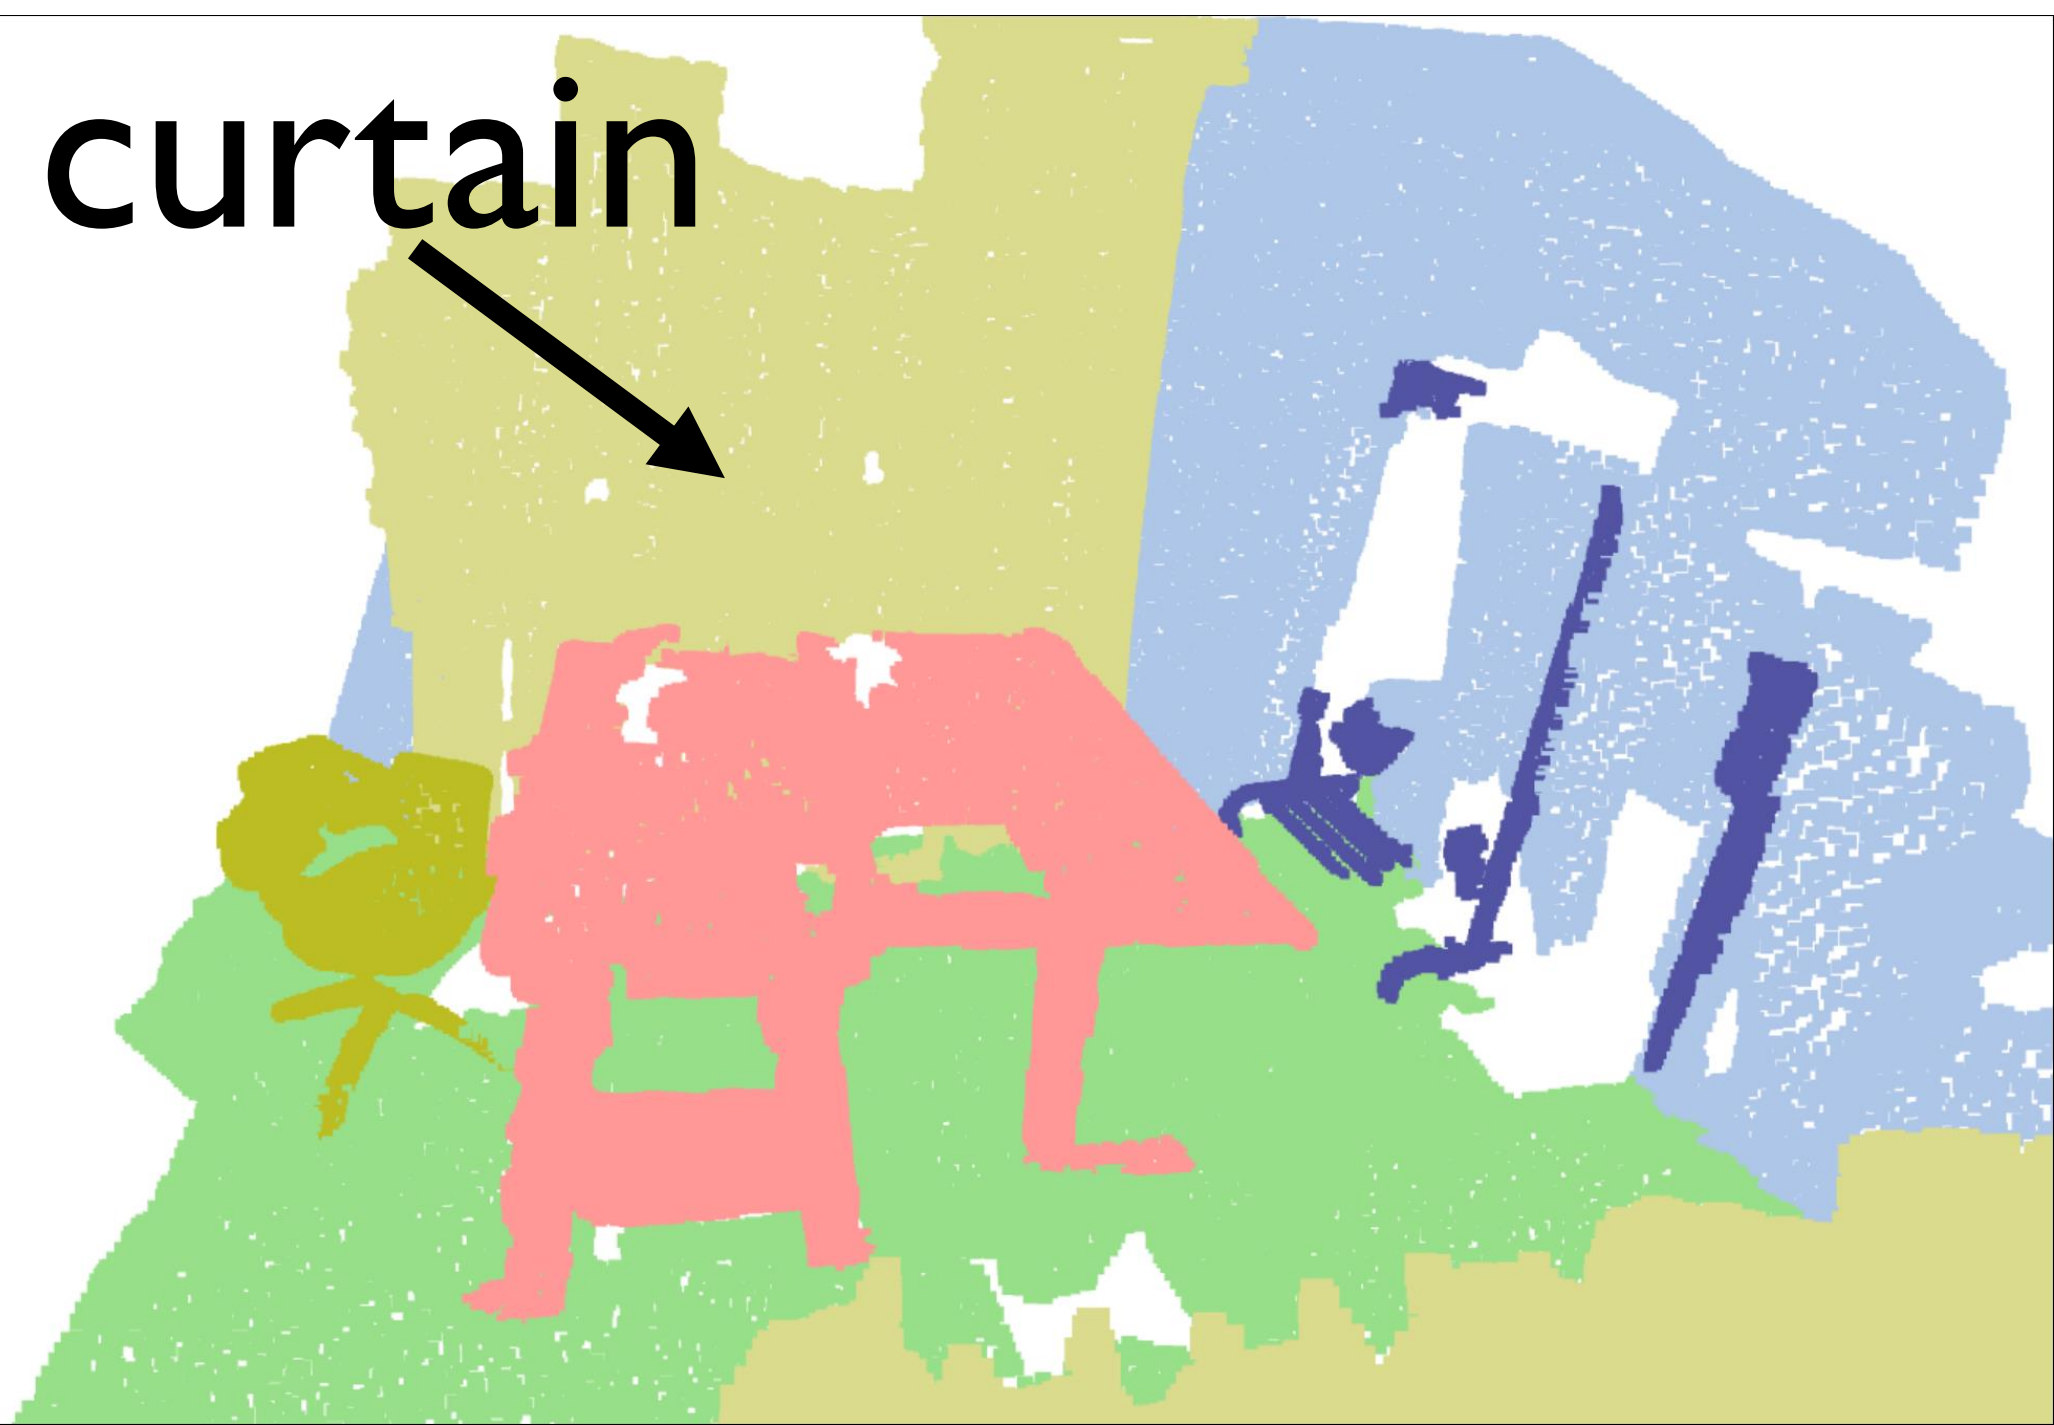



curtain

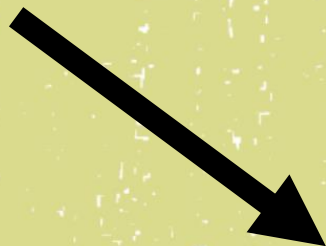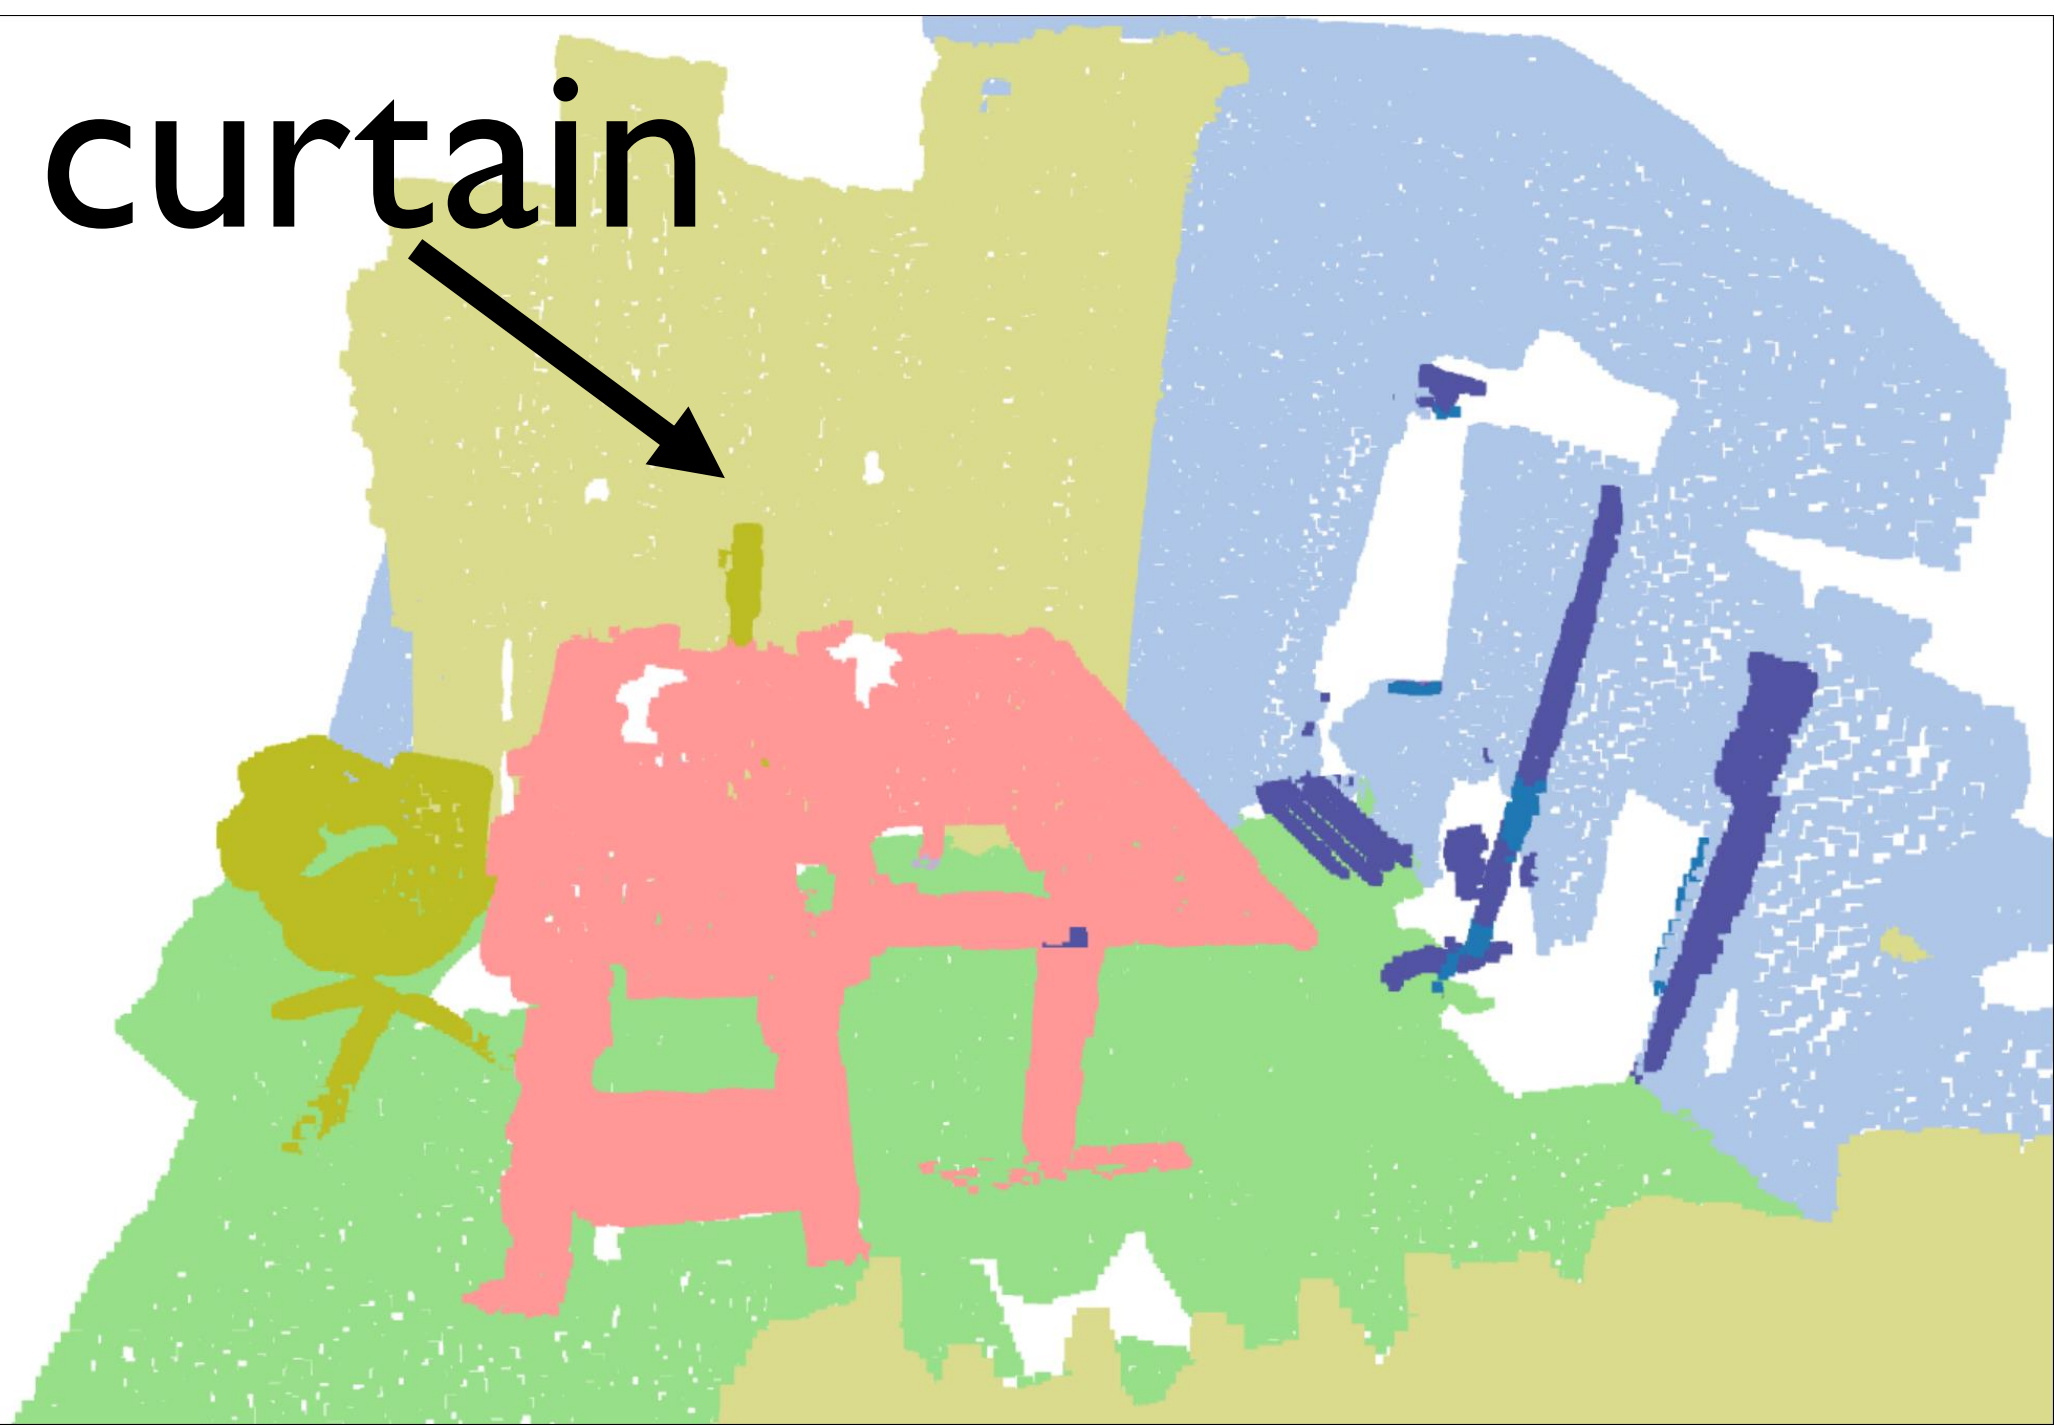

curtain

window

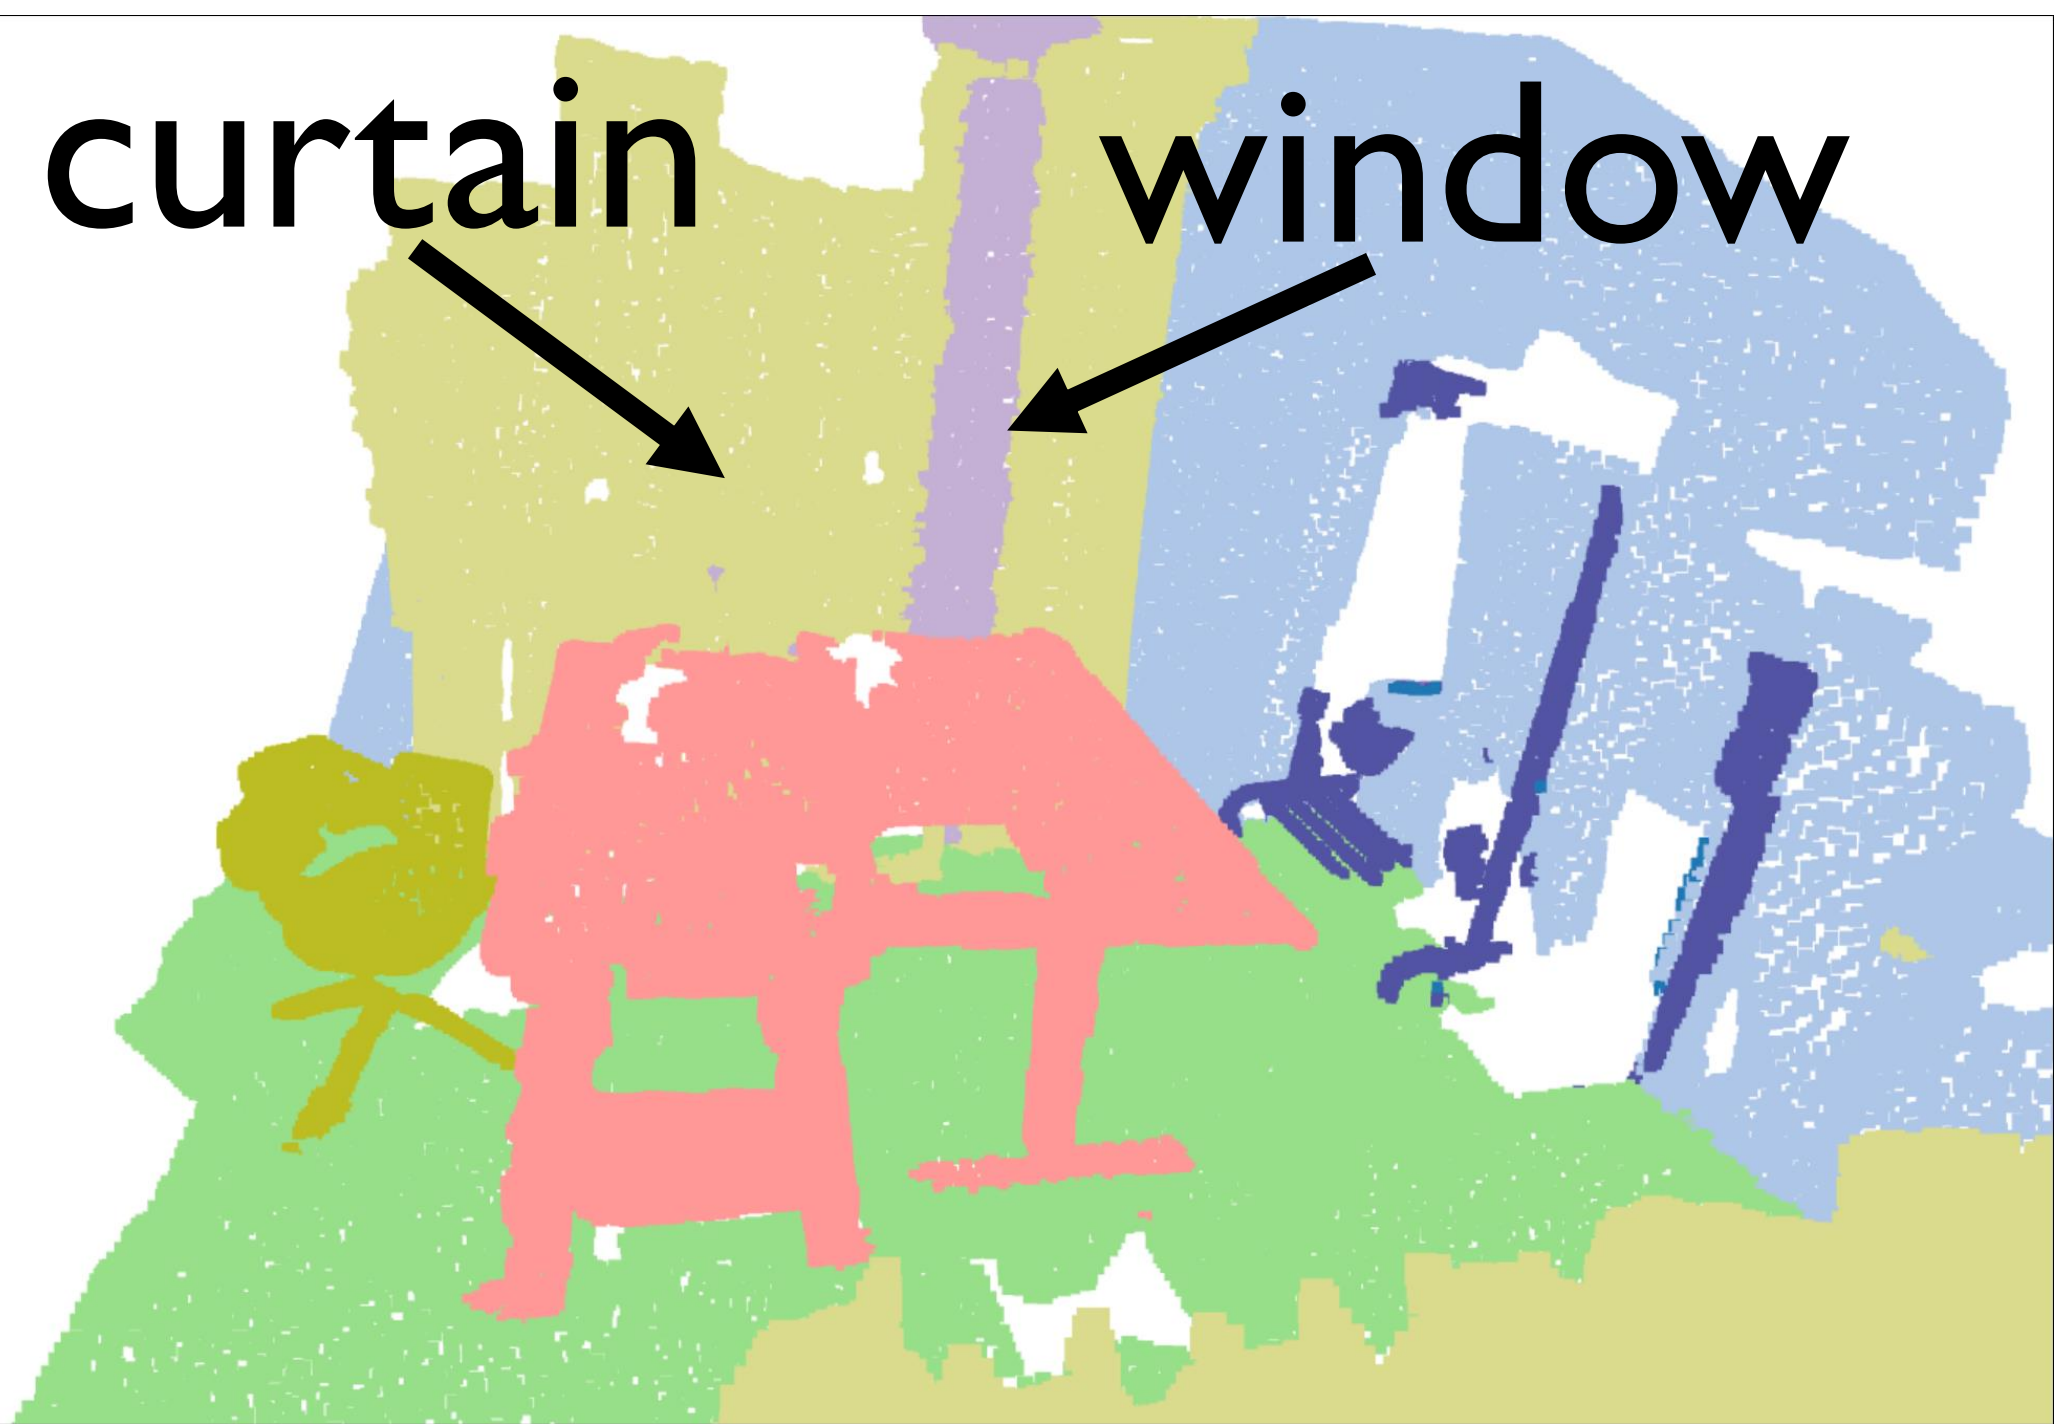

Supplement: Supplementary file 2 [file 288_oa0.9463763236999512.pdf]
