# Supplementary material for: Robust Point Cloud Segmentation with Noisy Annotations
Source: arXiv:2212.03242 source file (2022-12-06)
Supplement: Supplementary file 3 [file 309_from_relabeled.pdf]

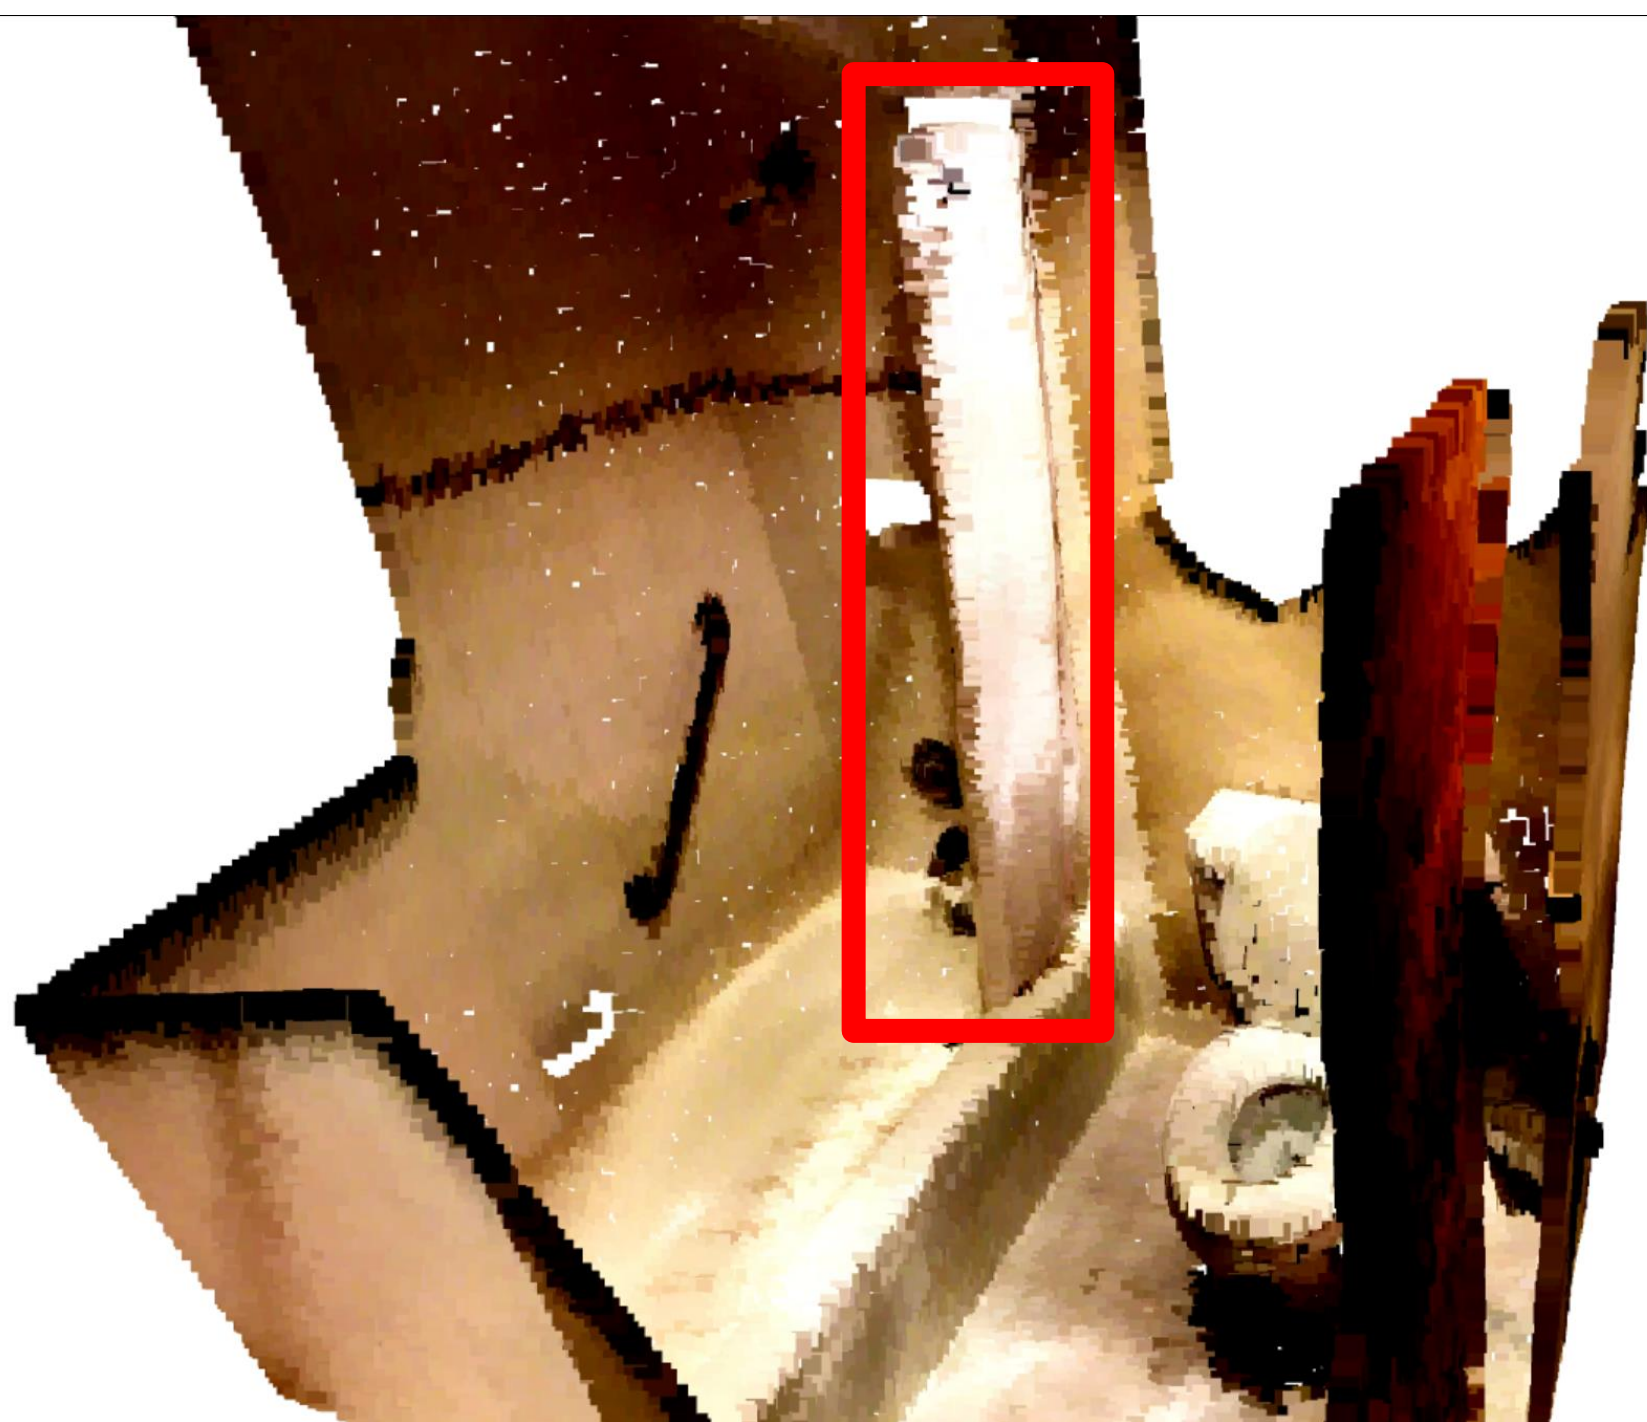

curtain

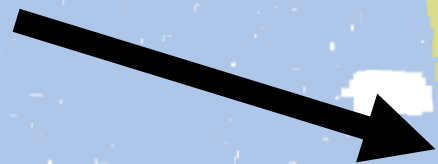

curtain

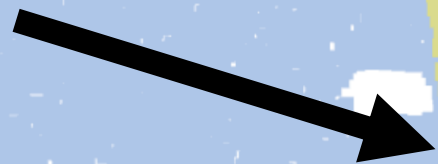

shower curtain

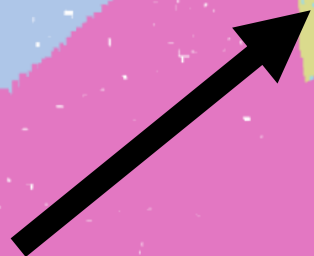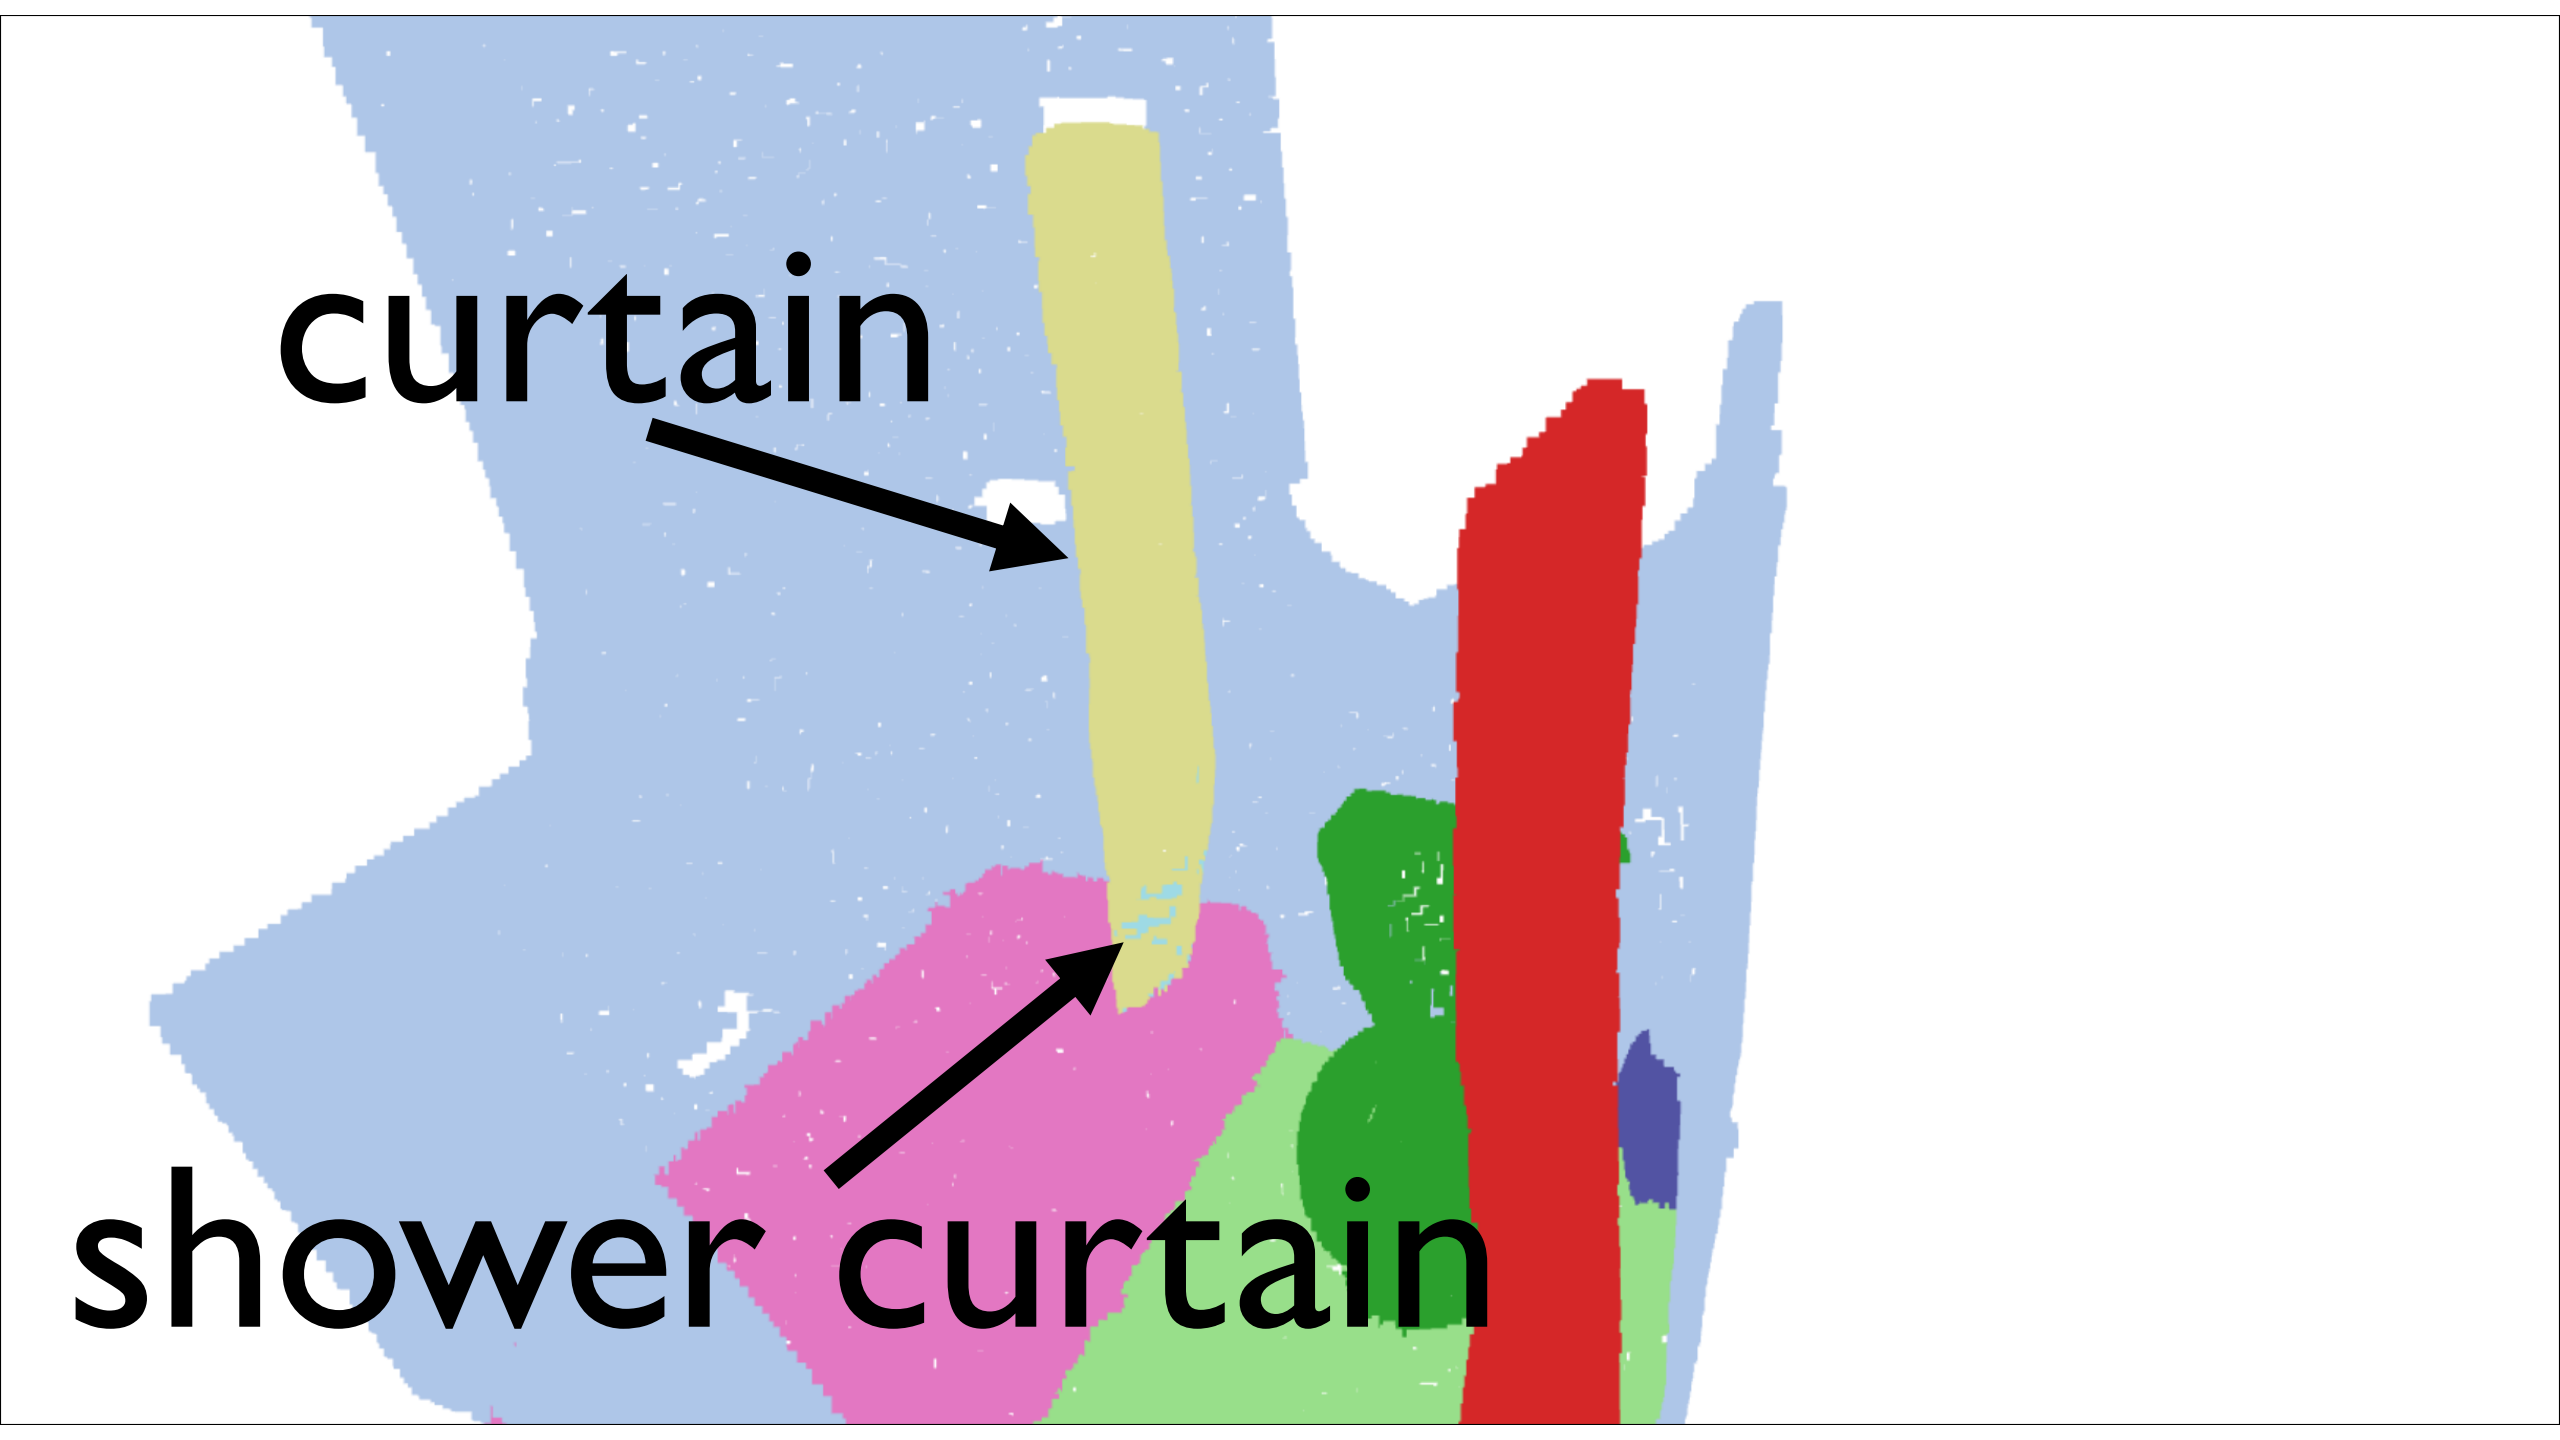

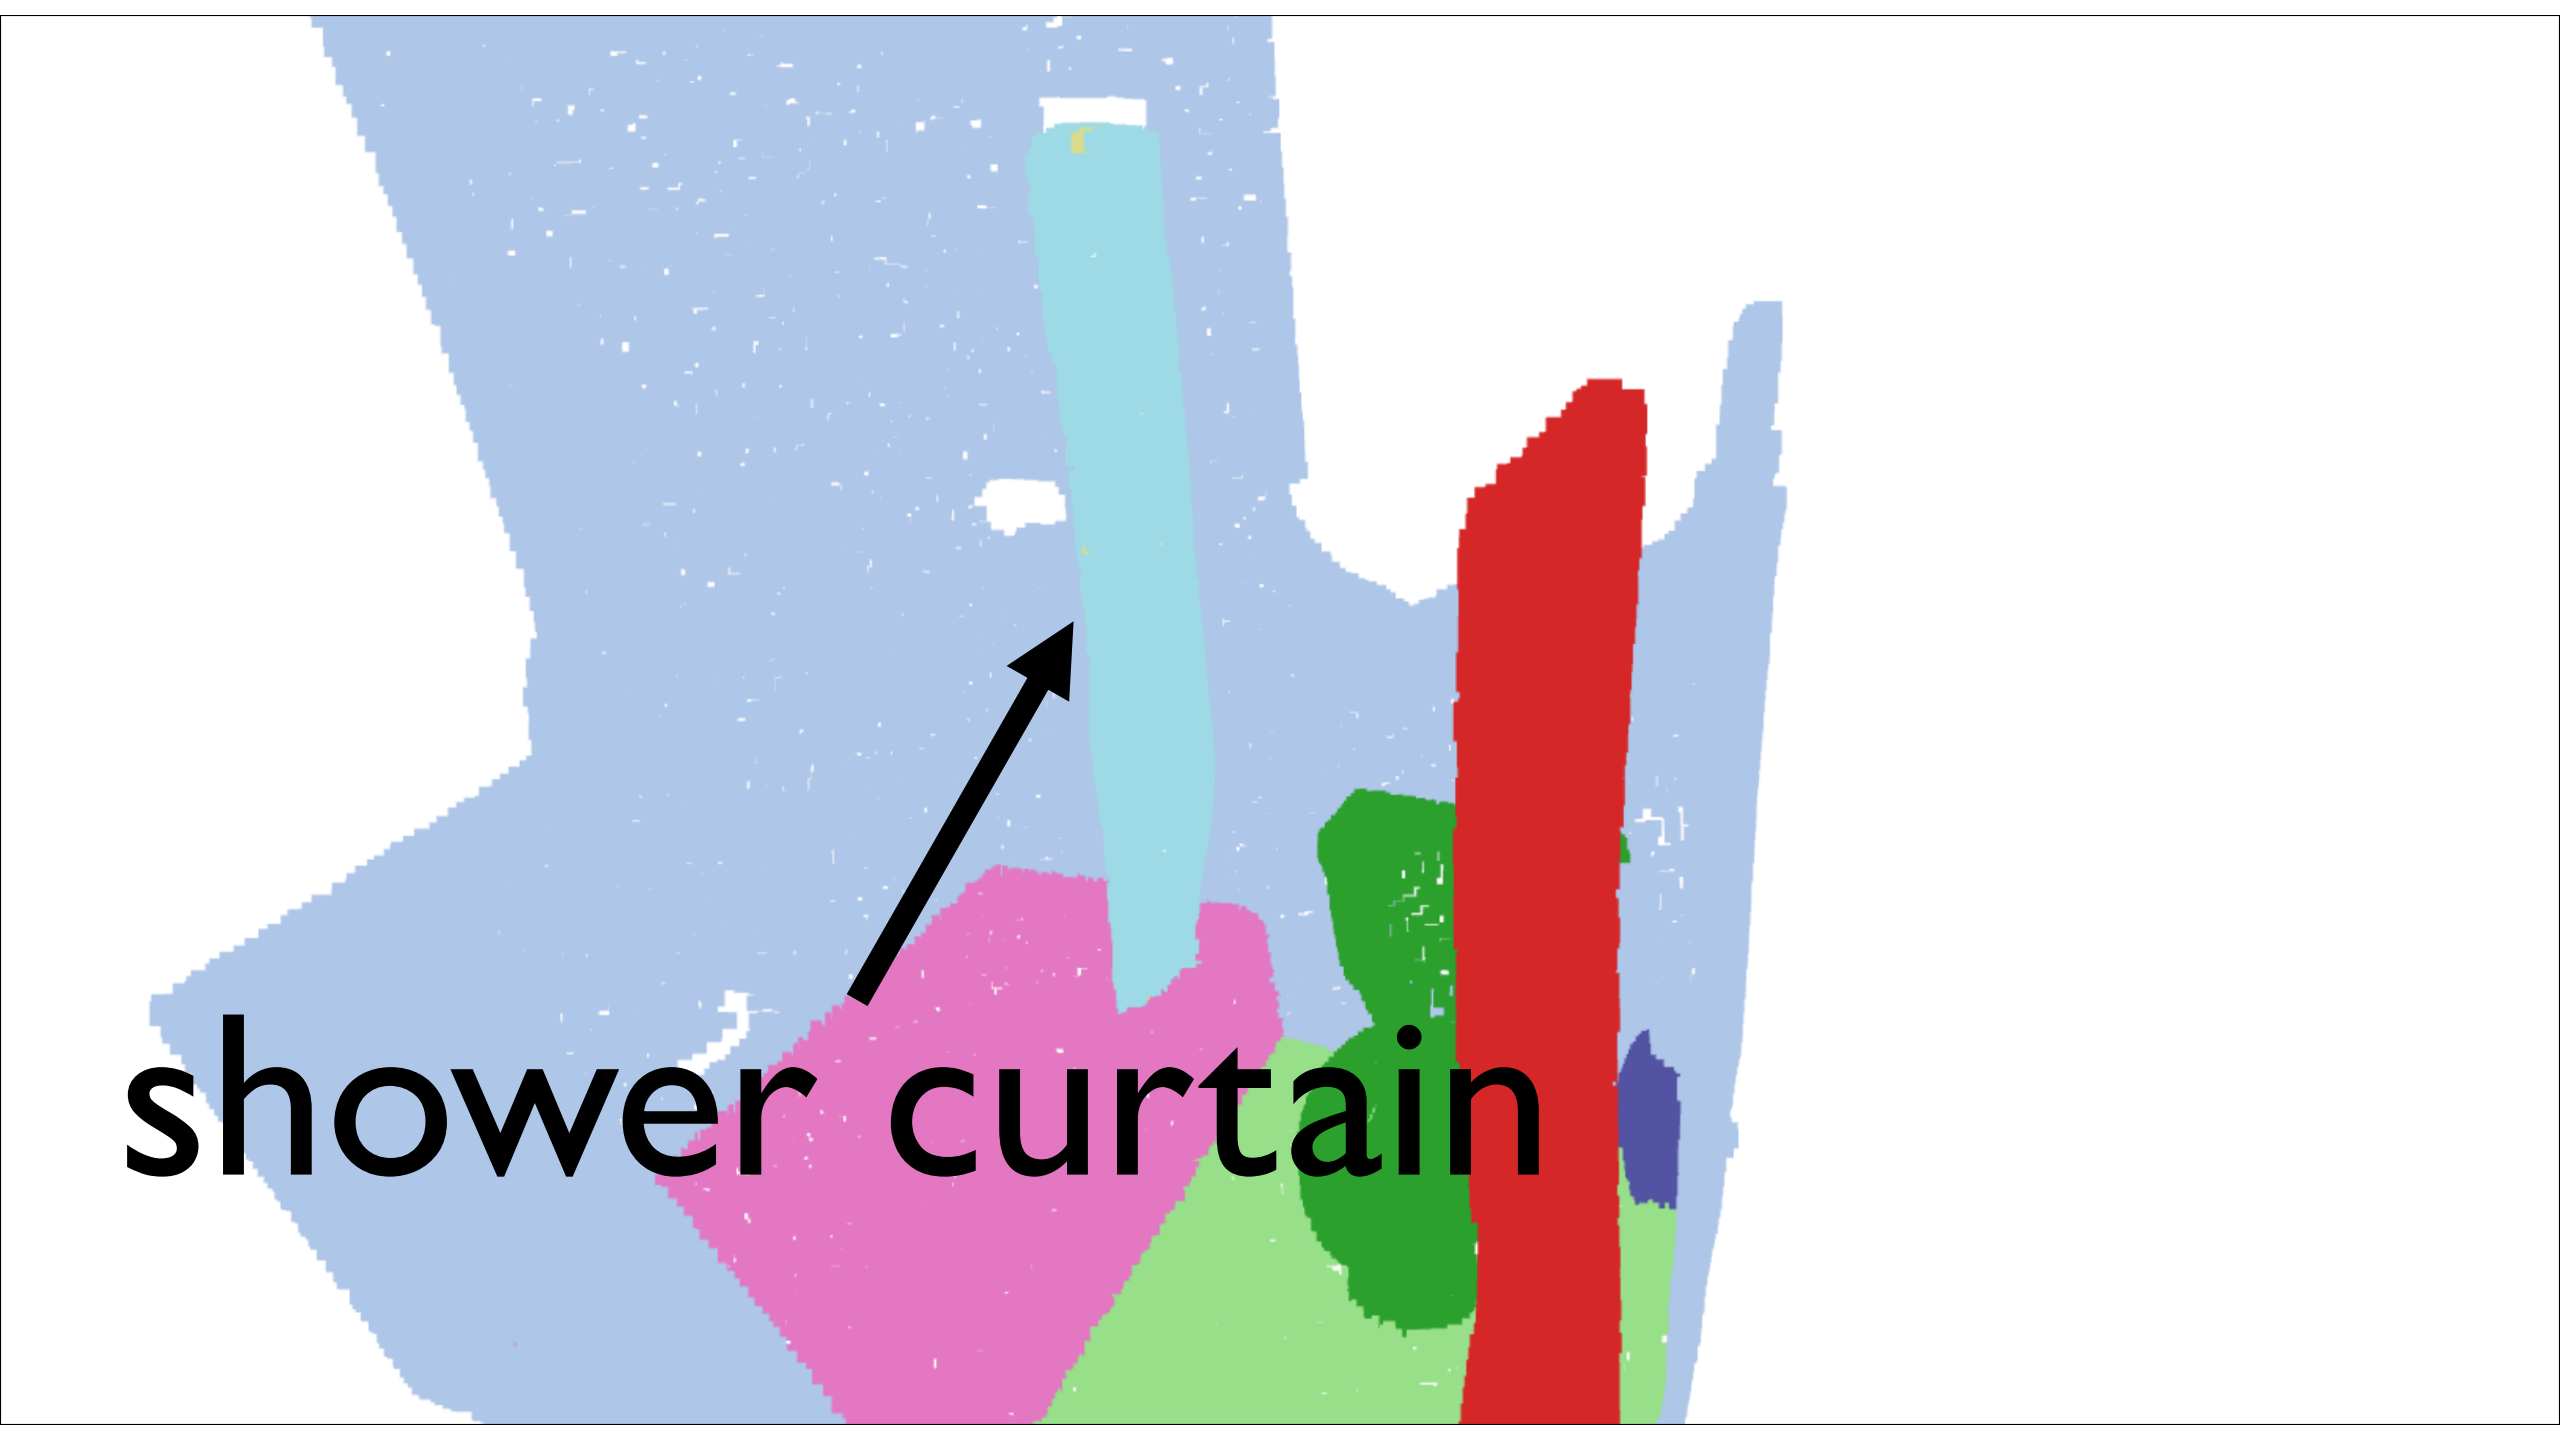

shower curtain
