# Supplementary material for: Robust Point Cloud Segmentation with Noisy Annotations
Source: arXiv:2212.03242 source file (2022-12-06)

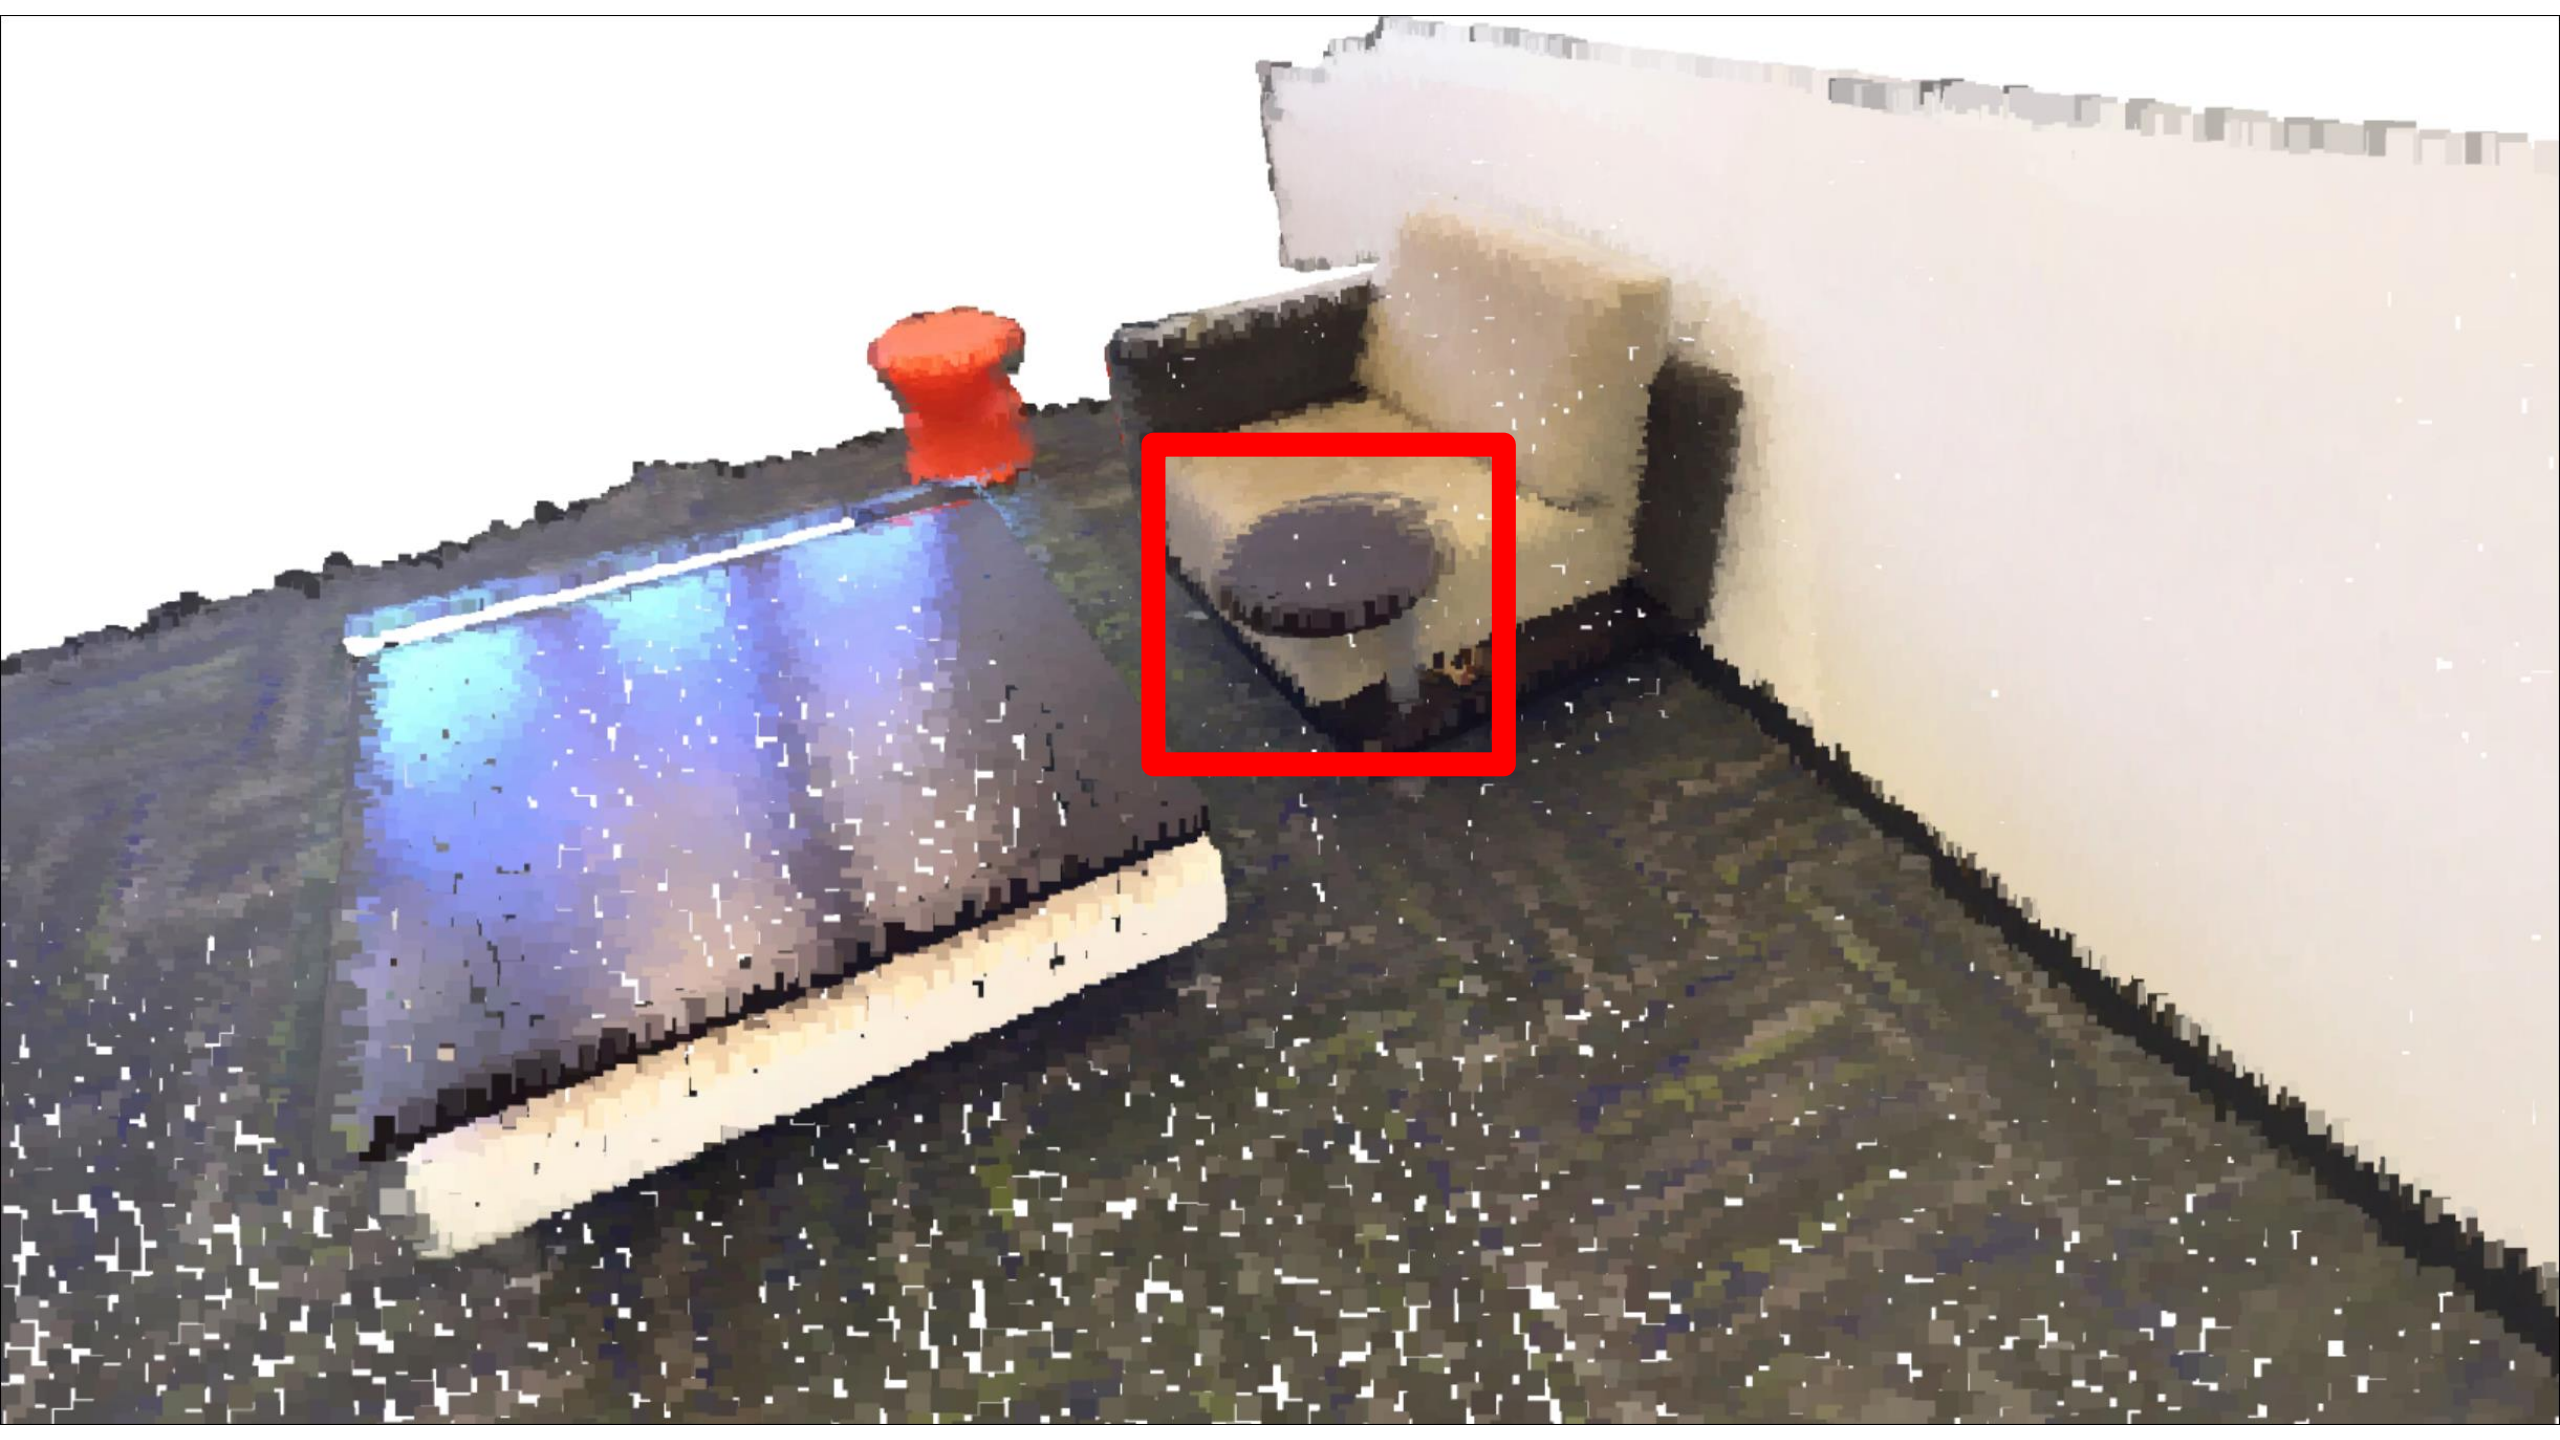

chair

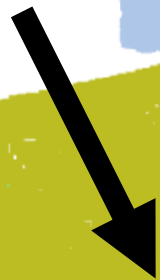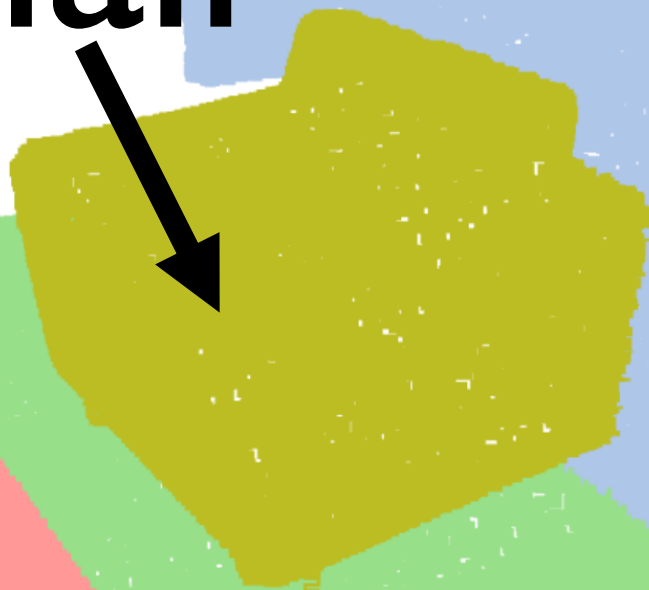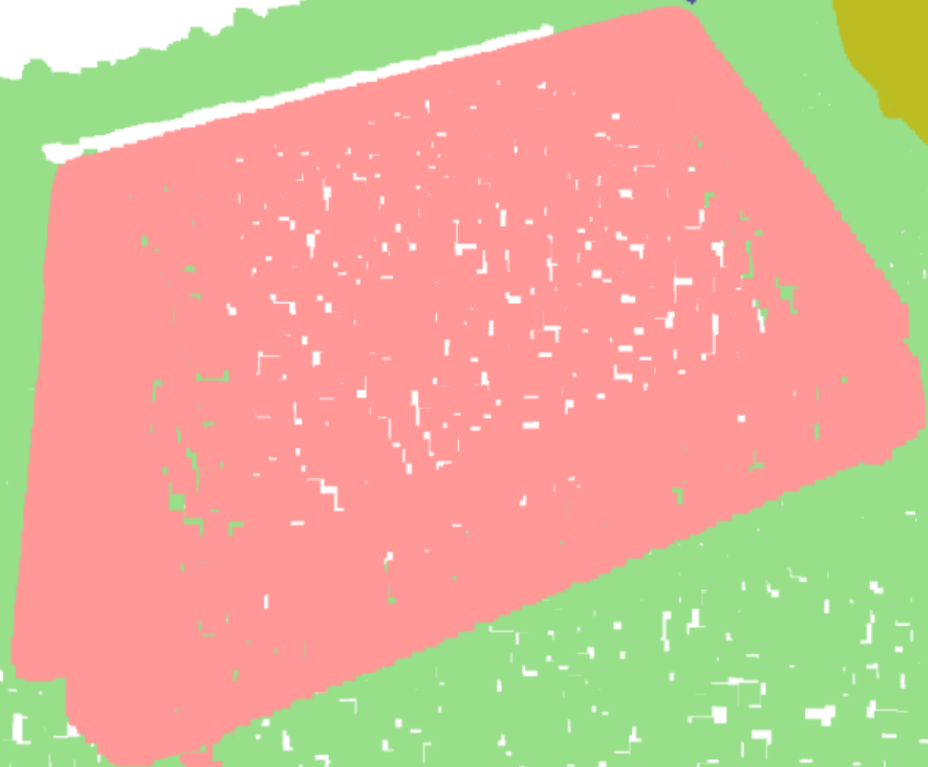

chair

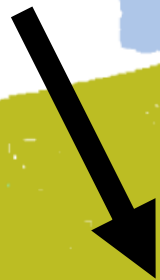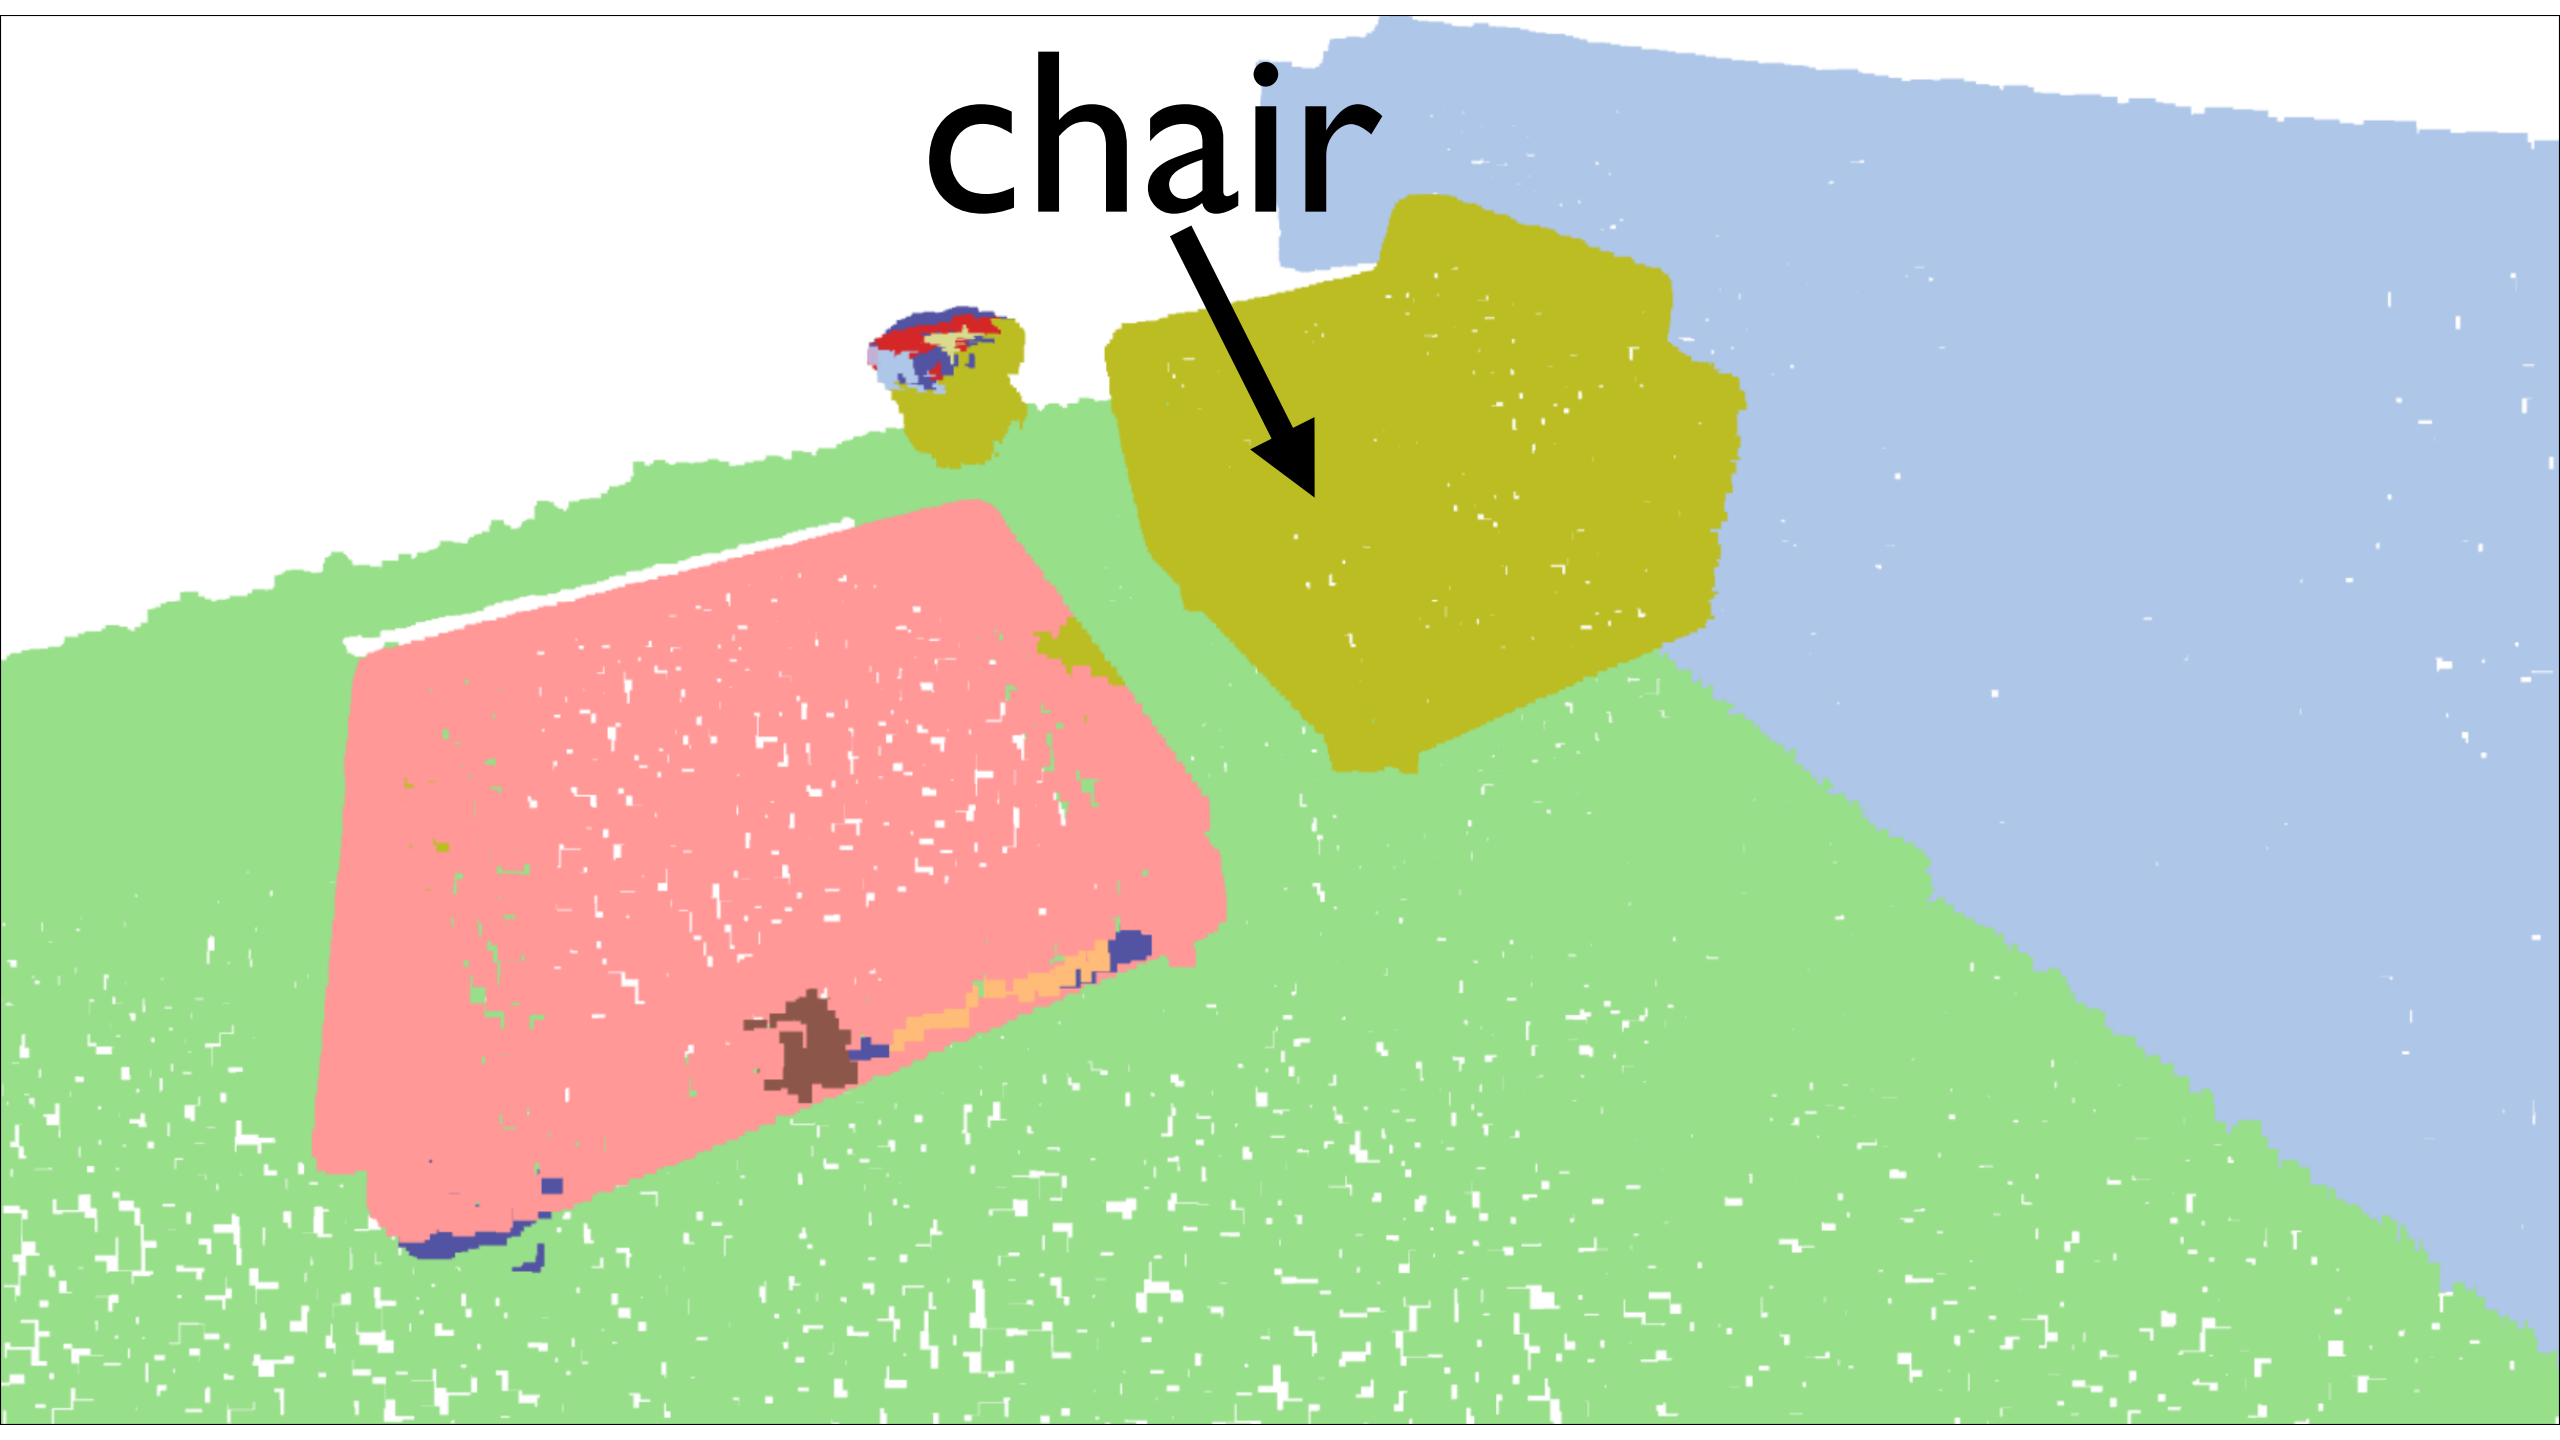

table chair

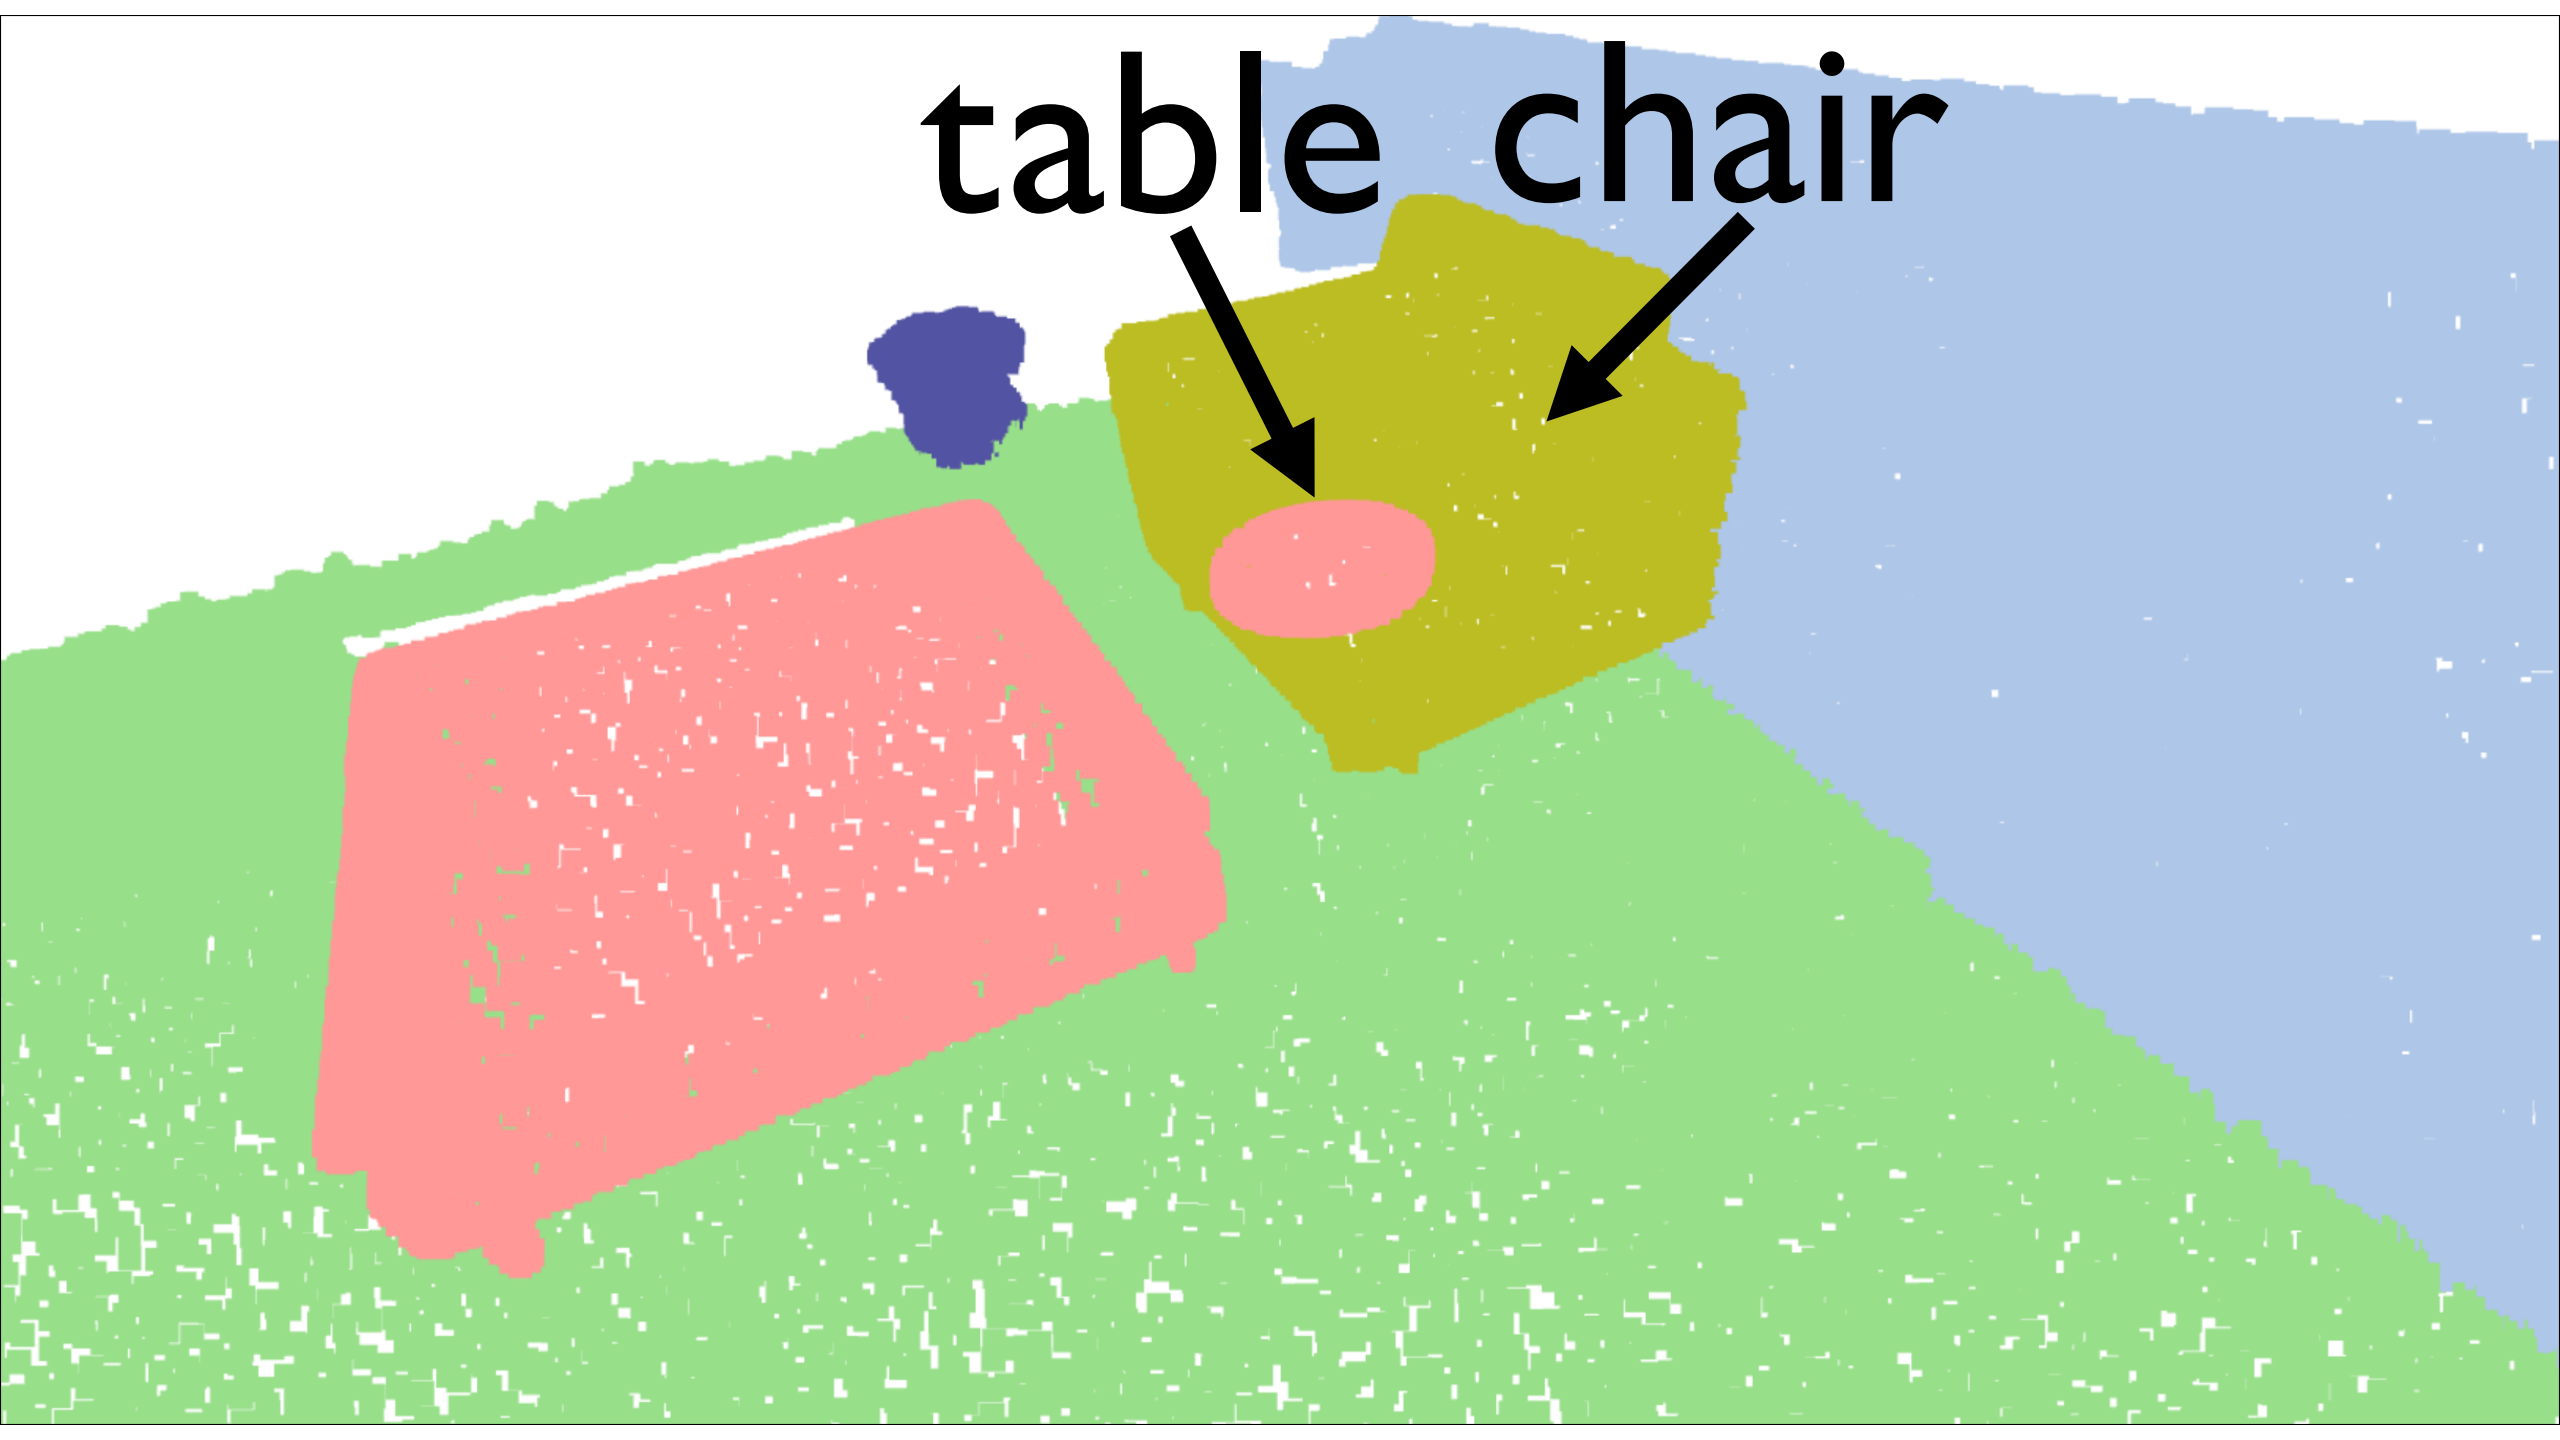

Supplement: Supplementary file 4 [file 59_oa0.9506_oa20.7511.pdf]
